# Supplementary material for: On the Paradox of Certified Training
Source: arXiv:2102.06700 source file (2022-10-12)
Supplement: Supplementary file 1 [file main_no_appendix.pdf]

---

# Certified Defenses: Why Tighter Relaxations May Hurt Training

---

Nikola Jovanović\*, Mislav Balunović\*, Maximilian Baader, Martin Vechev

Department of Computer Science

ETH Zurich, Switzerland

{nikola.jovanovic,mislav.balunovic,mbaader,martin.vechev}@inf.ethz.ch

## Abstract

Certified defenses based on convex relaxations are an established technique for training provably robust models. The key component is the choice of relaxation, varying from simple intervals to tight polyhedra. Paradoxically, however, training with tighter relaxations can often lead to worse certified robustness. The poor understanding of this paradox has forced recent state-of-the-art certified defenses to focus on designing various heuristics in order to mitigate its effects. In contrast, in this paper we study the underlying causes and show that tightness alone may not be the determining factor. Concretely, we identify two key properties of relaxations that impact training dynamics: continuity and sensitivity. Our extensive experimental evaluation demonstrates that these two factors, observed alongside tightness, explain the drop in certified robustness for popular relaxations. Further, we investigate the possibility of designing and training with relaxations that are tight, continuous and not sensitive. We believe the insights of this work can help drive the principled discovery of new and effective certified defense mechanisms.

## 1 Introduction

The increased use of deep learning in safety-critical applications has triggered significant interest in *certified defenses*: methods able to train provably robust models. One class of such techniques provides guarantees by leveraging different convex relaxations (e.g., CROWN-IBP [1], hBox [2]), that approximate the effect of network layers on the input specification. The main property of a relaxation is *tightness*, indicating how close it is to the possibly non-convex shape it approximates.

**The paradox of certified training** As tighter relaxations are generally more effective in certification of standard models, a natural belief is that tightness is also a favorable property when a relaxation is used for training as part of a certified defense. Surprisingly, several prior works [1, 3–6] have noticed that looser relaxations, that do not perform well for certification, in fact do allow for higher certified robustness after training with them. We illustrate this on a real model in Table 1, where for each relaxation we show its tightness and training score (certified robustness of the network at the end of certified training). We easily observe a paradox: *tighter relaxations obtain worse results*.

This was emphasized in prior work [1, 3–6], and strongly influenced the direction of the field of certified defenses. While some hypothesize that tighter relaxations introduce a more difficult optimization problem [5, 6], the underlying fundamental reasons for the paradox remain unclear. In light of this, recent advances mainly attempt to mitigate it in practice by improving the optimization problem through a training curriculum [3], a combination of several relaxations [1], or layerwise training [5]. However, the development of new relaxations effective for certified training seems to have reached a plateau. Gaining deeper insight into this phenomenon could restart progress and lead to major improvements in the design of certified defenses.

---

\*Equal contribution

Table 1: The paradox of certified training: *tighter methods obtain worse results*. Darker is better. CROWN-IBP (R) is the pure CROWN-IBP relaxation, as opposed to the complete certified defense. Training Score denotes certified robustness (in %). Tightness definition and more details in Section 3.

| Method                                 | Tightness | Training Score |
|----------------------------------------|-----------|----------------|
| Box / IBP [2, 3, 7]                    | 0.73      | 86.8           |
| hBox / Symbolic Intervals [2, 8]       | 1.76      | 83.7           |
| CROWN-IBP (R) [1]                      | 2.15      | 75.4           |
| DeepZ / CAP / FastLin / Neurify [9–12] | 3.00      | 69.8           |
| CROWN / DeepPoly [13, 14]              | 3.36      | 70.2           |

**This work** In this work we investigate the fundamental reasons for the paradox of certified training. We introduce two properties that impact certified training: we (i) observe that some relaxations lead to highly *discontinuous* losses during training, and (ii) find that some relaxations are more *sensitive* to changes in network parameters, resulting in a highly non-linear local loss landscape. While aiming to interpret the results in Table 1 purely from the perspective of tightness led to a seemingly contradictory conclusion, simultaneously considering continuity, sensitivity, and tightness provides a satisfying explanation and demystifies the paradox. Namely, the tighter relaxations in Table 1 are harmed by discontinuity or high sensitivity (both of which directly affect first-order methods typically used for training) and are thus unable to outperform Box. In light of these findings, we conduct a preliminary investigation into the possibility of designing relaxations with no unfavorable properties, and obtain promising initial results on a small network. Our hope is that the ideas presented in this work can guide the creation of new certified defenses based on novel relaxations and training schemes.

**Main Contributions** Our key contributions are:

- Two fundamental properties, continuity and sensitivity, that can greatly influence the success of a convex relaxation when used in certified training (Section 4).
- An extensive experimental evaluation, verifying that we can unravel the paradox of certified training by concurrently observing continuity, sensitivity, and tightness (Section 5.1).
- A preliminary small-scale investigation into the prospects of designing relaxations with no harmful properties, using a novel training setup based on implicit layers (Section 5.2).

## 2 Background and Related Work

We now discuss closely related work and provide the necessary background of convex relaxation-based neural network certification and certified training, presented within a framework [15] that captures common single neuron relaxations, thus simplifying analysis and comparison.

The discovery that neural networks are not robust to small input perturbations [16, 17] led to defenses based on adversarial training [18–20], which harden the model by training with adversarial examples. While adversarial defenses attain good empirical robustness, they lack robustness guarantees. An increasingly popular certification method are convex relaxations [9, 7, 10, 14, 21, 22] – a comprehensive exposition can be found in Salman et al. [15] – here, we only provide an overview needed to understand our work. We focus on *linear relaxations*, as they are scalable (e.g. can certify ResNet34 [23]), contrary to SDP [21, 22] which is limited to smaller networks, and even on these it is outperformed by linear relaxations [24, 25]. Other, prohibitively costly approaches, use multi-neuron relaxations [26, 27, 24, 25], or rely on SMT [28] or MILP [29] solvers. A fundamentally different approach, not the focus of our work, is randomized smoothing [30–32]. While more scalable, smoothing is probabilistic and introduces overhead at inference time, making it unsuitable for certain applications.

**Setting** We consider an  $L$ -layer feedforward ReLU network  $h = h_L \circ h_{L-1} \circ \dots \circ h_1$  with parameters  $\theta$ , where  $h_i : \mathbb{R}^{n_{i-1}} \rightarrow \mathbb{R}^{n_i}$  is the transformation applied at layer  $i$ . Let the network input be  $\mathbf{x}_0 \in \mathbb{R}^{n_0}$  and let  $\mathbf{x}_i := h_i \circ \dots \circ h_1(\mathbf{x}_0)$  be the result after layer  $i$ , for  $i \in [L]$ , where  $[L] := \{1, \dots, L\}$ . Each  $h_i$  is either a linear layer (dense or convolutional)  $\mathbf{x}_i = \mathbf{W}_i \mathbf{x}_{i-1} + \mathbf{b}_i$ , or a ReLU layer  $\mathbf{x}_i = \max(\mathbf{x}_{i-1}, 0)$ , where  $\max$  is applied componentwise. Further, we assume the two

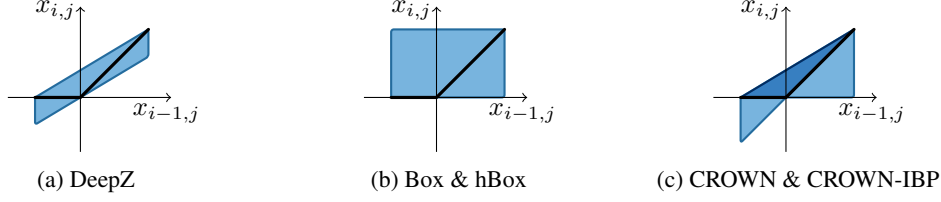

Figure 1: Illustration of unstable ReLU convex relaxations for methods introduced in Section 2.

layer types alternate, with  $h_1$  and  $h_L$  being linear. We focus on classification, where inputs  $\mathbf{x}_0$  are classified to one of  $n_L$  classes, based on the logit vector  $\mathbf{z} \equiv \mathbf{x}_L$ .

To certify robust classification to  $y$  in an  $\ell_\infty$  ball of radius  $\epsilon > 0$  around  $\mathbf{x}$ , we prove for every  $y' \neq y$

$$\mathbf{c}_{y'}^T \mathbf{z} < 0, \quad \mathbf{z} := h(\mathbf{x}_0), \quad \forall \mathbf{x}_0, \|\mathbf{x} - \mathbf{x}_0\|_\infty < \epsilon,$$

where  $\mathbf{c}_{y'} = \mathbf{e}_{y'} - \mathbf{e}_y$ , by upper bounding the left-hand side with a negative value.

**Convex relaxations** The certification with convex relaxations proceeds layer by layer, producing elementwise lower and upper bounds of  $\mathbf{x}_i$ ,  $\mathbf{l}_i \in \mathbb{R}^{n_i}$  and  $\mathbf{u}_i \in \mathbb{R}^{n_i}$  respectively. Starting from  $\mathbf{l}_0 = \mathbf{x} - \epsilon$  and  $\mathbf{u}_0 = \mathbf{x} + \epsilon$  we aim to obtain  $\mathbf{l}_L$  and  $\mathbf{u}_L$ , which directly yields the desirable upper bounds of  $(\mathbf{e}_{y'} - \mathbf{e}_y)^T \mathbf{z}$  for all  $y'$ , allowing us to verify the robustness property. To this end, all of the following methods maintain one upper and one lower linear bound for every neuron  $x_{i,j}$  of layer  $i$ :

$$\underline{\mathbf{a}}_{ij}^T \mathbf{x}_{i-1} + \underline{d}_{ij} \leq x_{i,j} \leq \overline{\mathbf{a}}_{ij}^T \mathbf{x}_{i-1} + \overline{d}_{ij}, \quad (1)$$

where  $\underline{\mathbf{a}}_{ij}, \overline{\mathbf{a}}_{ij} \in \mathbb{R}^{n_{i-1}}$  and  $\underline{d}_{ij}, \overline{d}_{ij} \in \mathbb{R}$  for all  $j \in [n_i]$ . Excluding the *Box* relaxation, all methods use  $x_{i,j} = (\mathbf{W}_i \mathbf{x}_{i-1})_j + b_{i,j}$  for linear layer bounds,  $x_{i,j} = 0$  if  $u_{i-1,j} \leq 0$  and  $x_{i,j} = x_{i-1,j}$  if  $l_{i-1,j} \geq 0$  for stable ReLU bounds, and calculate  $\mathbf{l}_i$  and  $\mathbf{u}_i$  using *backsubstitution* introduced next. Unstable ReLU ( $l_{i-1,j} < 0 < u_{i-1,j}$ ) bounds are method-specific and can depend on  $\mathbf{l}_{i-1}$  and  $\mathbf{u}_{i-1}$ .

**Backsubstitution** Starting with the bound for  $x_{i,j} \leq \overline{\mathbf{a}}_{ij}^T \mathbf{x}_{i-1} + \overline{d}_{ij}$ , we substitute  $\mathbf{x}_{i-1}$  by replacing each  $x_{i-1,j'}$  with its respective bound  $\overline{\mathbf{a}}_{i-1,j'}^T \mathbf{x}_{i-2} + \overline{d}_{i-1,j'}$  if  $(\overline{\mathbf{a}}_{ij})_{j'}$  is positive and with its lower bound otherwise. This can be repeated recursively through the layers until we arrive at constraints of the form

$$\underline{\mathbf{p}}_j^T \mathbf{x}_0 + \underline{q}_j \leq x_{i,j} \leq \overline{\mathbf{p}}_j^T \mathbf{x}_0 + \overline{q}_j, \quad (2)$$

where  $\underline{\mathbf{p}}_j^T, \overline{\mathbf{p}}_j^T \in \mathbb{R}^{n_0}$  and  $\underline{q}_j, \overline{q}_j \in \mathbb{R}$  for all  $j \in [n_i]$ . Here, we can in turn substitute the appropriate side of  $\mathbf{l}_0 \leq \mathbf{x}_0 \leq \mathbf{u}_0$  for each element in  $\mathbf{x}_0$ , to obtain an upper bound  $\mathbf{l}_{i,j}$  on  $x_{i,j}$  solely w.r.t. the bounds of  $\mathbf{x}_0$ . We provide more details of this procedure in Appendix A.

Note that while some of the relaxations have more efficient implementations, they produce the same outputs as our formulation. We use this formulation as it allows us to capture all of the needed relaxations and further, our results are conceptual and hold for any implementation. We also note that for each set of equivalent relaxations, we choose one name and use it in the remainder of the paper.

**DeepZ** The *DeepZ* relaxation [10] is equivalent to *CAP* [9], *Fast-Lin* [11], and *Neurify* [12]. It uses the following relaxation for unstable ReLUs (Figure 1a):

$$\lambda x_{i-1,j} \leq x_{i,j} \leq \lambda x_{i-1,j} - \lambda l_{i-1,j}, \quad \text{where } \lambda := u_{i-1,j} / (u_{i-1,j} - l_{i-1,j}).$$

**Box/hBox** The *Box* [2, 7] or *IBP* [3] relaxation uses interval arithmetic instead of backsubstitution, ignoring other dependencies. For linear layers, the upper bound (similarly for the lower bound) is  $(\mathbf{W}_i \mathbf{h}_{i-1})_j + b_{i,j}$  where  $h_{i-1,j} = u_{i-1,j}$  if the corresponding element of  $\mathbf{W}_i$  is positive, and  $h_{i-1,j} = l_{i-1,j}$  otherwise. For ReLU, it uses  $\text{ReLU}(l_{i-1,j}) \leq x_{i,j} \leq \text{ReLU}(u_{i-1,j})$  (Figure 1b). The relaxation *hBox* is an instantiation of a *hybrid zonotope* [2], also called *symbolic interval* in Wang et al. [8]. It uses the same bounds as *Box*,  $0 \leq x_{i,j} \leq u_{i-1,j}$ , for unstable ReLU, replacing  $x_{i,j}$  with these bounds in the rest of backsubstitution. For linear and stable ReLUs, as with all other methods except *Box*, it uses  $x_{i,j} = (\mathbf{W}_i \mathbf{x}_{i-1})_j + b_{i,j}$  and  $x_{i,j} = x_{i-1,j}$  ( $x_{i,j} = 0$ ), respectively.

**CROWN/CROWN-IBP** CROWN [13] and DeepPoly [14] have the same upper bound as DeepZ for unstable ReLUs, but choose the lower bound adaptively:  $0 \leq x_{i,j}$  if  $-l_{i-1,j} \geq u_{i-1,j}$ , or  $x_{i-1,j} \leq x_{i,j}$  otherwise (Figure 1c). CROWN-IBP [1] is a variant which efficiently computes  $l_i$  and  $u_i$  using Box at all layers except the last, which uses CROWN and performs a full backsubstitution.

**Certified training** While adversarial training improves empirical robustness, certified robustness usually remains low (regardless of the certification method), a common observation also reaffirmed in Appendix B. Recent work on *certified training* addresses this issue and aims to produce networks amenable to certification by incorporating the chosen certification method into the training procedure [9, 2, 1, 3, 33, 34]. The training proceeds by constructing the worst case logit  $\hat{z}$  where  $\hat{z}_y = l_{L,y}$  and  $\hat{z}_{y'} = u_{L,y'}$  for all  $y' \neq y$ , minimizing the corresponding cross-entropy loss  $\mathcal{L}_{CE}(\hat{z}, y)$ . This loss is often combined with the standard cross-entropy  $\mathcal{L}_{CE}(z, y)$  using a tradeoff parameter  $\kappa$ .

While all of the above certification methods can be used in certified training, which greatly improves over adversarial defenses, the certified robustness achieved so far is still limited and far from the theoretical possibilities – see Baader et al. [35] which proves that Box-certified networks are universal approximators. We elaborate on the most notable practical limitation of certified training in Section 3.

### 3 Paradox: tighter relaxations hurt certified training

We now discuss tightness of relaxations, as well as a well known observation that training with tighter relaxations can lead to worse certified robustness, limiting the applicability of certified defenses.

**Tightness should help training** Given a network certifiably robust around  $x$ , the success of certification depends on the *tightness* of the chosen relaxation, i.e., the tightness of its bounds. While it is not always possible to provably compare the tightness of methods, there is a consistent empirical understanding of their relative tightness. We illustrate this in Figure 2, where we compare the *certified robustness (CR) curve* of each relaxation on a fixed MNIST network, obtained via standard training.

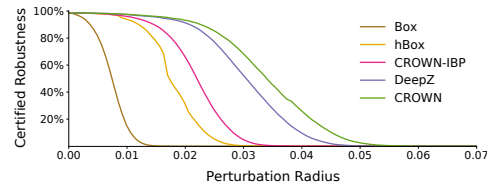

Figure 2: CR curves of convex relaxations on a convolutional network trained on MNIST.

Intuitively, tighter relaxations should produce better output bounds for most networks, as in Figure 2. For some relaxations, such as Box and hBox, we can in fact prove (see Appendix C) that for *any* network parameters, the tighter relaxation certifies more inputs. Clearly, tightness should indeed be a favorable property for certified training, as tighter relaxations can have a better global optimum.

**Tighter relaxations obtain worse results** Surprisingly, while one would expect for tighter methods used in training to produce higher certification rates, it is well established [1, 3–6] that this is in fact not the case in practice, and tighter methods obtain worse results. Most notably, Gowal et al. [3] observed that Box training often outperforms training with DeepZ which is (empirically) tighter. We refer to this phenomenon as *the paradox of certified training*: tighter relaxations obtain worse results.

We illustrate this in Table 1. In the left column, we report *CR-AUC*, the area under the CR curve of each method after standard training (calculated from Figure 2), as a way to quantify tightness. Note that CR-AUC depends on the network choice and the training procedure, but can be used to compare tightness across methods. In the right column, we report the certified robustness on MNIST with  $\epsilon_{test} = 0.3$  after certifiably training the same network with each method. More details and additional tightness experiments are given in Appendix B. Note that we use CROWN-IBP (R) to denote the use of the pure CROWN-IBP relaxation for both training and certification ( $\beta : 1 \rightarrow 1$  mode in [1]), as opposed to the state-of-the-art defense usually referred to as CROWN-IBP, which combines the CROWN-IBP (R) loss with the IBP loss in training, and uses IBP to certify ( $\beta : 1 \rightarrow 0$  mode in [1]).

The intuition around tightness suggests that existence is not the reason for the paradox as for a fixed architecture, e.g., the best network for (tighter) hBox is at least as good as the one for Box. Further, while prior work hypothesized that tighter relaxations over-regularize the network [1], yield hard optimization problems [5] or simply stated that they unexpectedly underperform [3, 4], the only deeper study so far has been the recent work of Lee et al. [6]. However, their theory is limited to continuous

relaxations, so it does not apply and cannot explain the results of hBox, CROWN, CROWN-IBP, as these, being discontinuous (Section 4.1), violate their Lipschitz continuity assumption.

## 4 Analysis of certified training: continuity and sensitivity

In this section we investigate the fundamental reasons behind the paradox discussed in Section 3. While tightness was the sole focus of most prior work, the paradox suggests that this is insufficient to paint a complete picture in the case of certified training, where relaxations are used inside first-order optimization. Concretely, we introduce two key properties of convex relaxations, *continuity* and *sensitivity*, and use these alongside tightness to analyze certified training and resolve the paradox.

### 4.1 Continuity of convex relaxations

While convex relaxations represent layer constraints as convex sets, the loss optimized during training is not necessarily convex w.r.t. network weights. Moreover, we observe that some relaxations introduce a *discontinuous* loss landscape, harming first-order optimization as the gradient values near the discontinuity do not provide *any* information about the function behavior after the discontinuity (see Section 4.4). We show that CROWN, CROWN-IBP, and hBox all suffer from this issue.

We focus on the discontinuity of the output layer lower bounds  $l_L$ , treating each  $l_{L,j}$  as a function of the network weights. Note that all findings can be easily extended to the actual loss function  $\mathcal{L}_{CE}(\hat{z}, y)$ . We construct a minimal example necessary to produce the discontinuities: a 3-layer network with input  $x_{0,1} \in [-1, 1]$ , linear layer  $x_{1,1} = x_{1,2} = x_{0,1} + w$  where  $w$  is the only network parameter, ReLU layer  $x_{2,1} = \text{ReLU}(x_{1,1})$ ,  $x_{2,2} = \text{ReLU}(x_{1,2})$ , and the output layer given as  $x_{3,1} = x_{2,2} + 1$  and  $x_{3,2} = x_{2,2} - x_{2,1}$ . The discontinuities on this example are shown in Figure 3.

**Discontinuity of CROWN/CROWN-IBP** For CROWN, the discontinuities arise due to its adaptive choice of the lower bound for unstable ReLUs (Figure 1c), used as a heuristic to tighten the bounds. In our minimal example, assume we use CROWN to compute the lower bound  $l_{3,1}$  of  $x_{3,1}$ . For  $w \in [-1, 1]$ , the ReLUs are unstable with the preactivation range  $[-1 + w, 1 + w]$ . Thus, for  $w \in [-1, 0]$ , as  $-l_{2,1} \geq u_{2,1}$ , CROWN picks the lower bound  $x_{2,1} \geq 0$  so  $l_{3,1} = 1$ , and for  $w \in (0, 1]$  the lower bound  $x_{2,1} \geq x_{1,1}$  so  $l_{3,1} = w$ . This creates a discontinuity when  $-l_{2,1} = u_{2,1}$ , i.e., at  $w = 0$ . This implies the discontinuity of CROWN-IBP as it uses CROWN for its final bounds.

**Discontinuity of hBox** The discontinuities of hBox appear when ReLUs transition between unstable and positive stable cases, and are caused by hBox switching from simple Box bounds (Figure 1b), to directly exploiting the tight relation  $x_{i,j} = x_{i-1,j}$ . Assume we are computing  $l_{3,2}$ . For  $w \in (-1, 1)$ , the ReLUs are unstable, so we use Box bounds  $0 \leq x_{2,j} \leq u_{1,j} = 1 + w$  for  $j \in \{1, 2\}$ , obtaining  $l_{3,2} = -1 - w$ , which approaches  $-2$  as  $w$  approaches 1. However, for  $w \geq 1$ , we tighten the bound using  $x_{2,j} = x_{1,j}$ , resulting in  $l_{3,2} = 0$ , thus a discontinuity when  $l_{2,1} = l_{2,2} = 0$ , i.e., at  $w = 1$ .

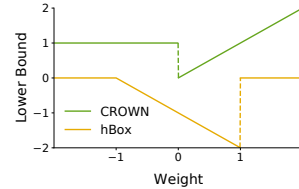

Figure 3: Discontinuity of CROWN and hBox.

As our example shows that only a few neurons are sufficient to produce a discontinuity, large networks are expected to have many such discontinuities, that can appear at any ReLU neuron  $x_{i,j}$ , whenever  $-l_{i-1,j} = u_{i-1,j}$  (for CROWN) or  $l_{i-1,j} = 0$  (for hBox). Backsubstitution accumulates their effect, creating an unfavorable landscape, as demonstrated in practice on a realistic network in Section 4.3.

**Continuity of other relaxations** The remaining two previously introduced relaxations, Box and DeepZ, are always continuous, as formalized in the following theorem (full proof in Appendix D.1):

**Theorem 1.** *The output bounds  $l_{L,j}$  of Box and DeepZ are continuous w.r.t network parameters  $\theta$ .*

*Proof Sketch.* For Box,  $l_i$  and  $u_i$  depend only on the previous layer, and the relationships used to derive them are either linear or ReLU, both continuous. For DeepZ, the key step is proving that the ReLU relaxation bounds are continuous in points where the ReLU changes stability. Recall that the unstable case bounds are  $\lambda x_{i-1,j}$  and  $\lambda x_{i-1,j} - \lambda l_{i-1,j}$ , where  $\lambda = u_{i-1,j} / (u_{i-1,j} - l_{i-1,j})$ . Then, as  $l_{i-1,j} \rightarrow 0$ ,  $\lambda \rightarrow 1$  and as  $u_{i-1,j} \rightarrow 0$ ,  $\lambda \rightarrow 0$ . For both, the unstable case bounds (in the limit) match the stable case ones; therefore, there is no discontinuity.  $\square$

## 4.2 Sensitivity of convex relaxations

Next, we analyze how a small change in weights affects the output loss of a given convex relaxation. Concretely, we measure the degree of change in the output when the *first* layer weights are shifted by  $\delta$  in the gradient direction. To capture this, we define a set of rational functions of  $\delta$  as  $R_N(\delta) = \{p(\delta)/q(\delta) \mid p(\delta), q(\delta) \in P_N(\delta)\}$ , where  $P_N(\delta)$  denotes the polynomials of degree up to  $N$ . Note that  $P_N(\delta) \subseteq R_N(\delta)$ . We say that some neuron  $x_{i,j}$  is in the set  $P_N(\delta)$  (or  $R_N(\delta)$ ) if that set contains both  $l_{i,j}$  and  $u_{i,j}$ , now treated as functions of  $\delta$  where  $\delta = 0$  corresponds to the concrete  $l_{i,j}$  and  $u_{i,j}$  used in Section 2. Everything else is treated as a constant. Recall that during backsubstitution for  $x_{i,j}$ , all encountered  $x_{i',j'}$  are *variables*, repeatedly replaced with bound expressions from Equation 1, until we reach Equation 2 and obtain linear expressions for  $l_{i,j}$  and  $u_{i,j}$ . If the output neurons of the network are in  $R_N(\delta)$ , we say that the *sensitivity* of a relaxation is  $N$ . As before, while we focus on  $\mathcal{L}_L$ , the conclusions can be extended to the actual loss. We always consider the worst case w.r.t. all bound choices and ReLU stability, and assume all layers are of size  $M$ . Sensitivity is an undesirable property of a relaxation, as it introduces a complex loss landscape that hinders optimization, as further explained in Section 4.4.

**Computing the sensitivity** As the first layer is linear, we see that for all relaxations,  $x_{1,j}$  are in  $P_1(\delta)$ . To compute the sensitivity of a relaxation, we sequentially analyze the effect of each layer.

**Box/hBox** For Box, assume that at layer  $i$ , all  $x_{i-1,j}$  are in  $P_N(\delta)$ . For ReLU, as  $u_{i,j} = \text{ReLU}(u_{i-1,j})$  (same for  $l_{i,j}$ ),  $x_{i,j}$  are also in  $P_N(\delta)$ . For a linear layer, as  $l_{i,j}$  and  $u_{i,j}$  are linear combinations of elements of  $\mathbf{u}_{i-1}$  and  $\mathbf{l}_{i-1}$ ,  $x_{i,j}$  again stay in  $P_N(\delta)$ . Thus, all network neurons are in  $P_1(\delta) \subseteq R_1(\delta)$  so the sensitivity of Box is 1. For hBox, the only difference are the linear layers, where now  $x_{i,j} = (\mathbf{W}_i \mathbf{x}_{i-1})_j + b_{i,j}$ . As a linear combination of the elements of  $P_N(\delta)$  stays in  $P_N(\delta)$ , we again conclude that all neurons stay in  $P_1(\delta)$  and the sensitivity of hBox is also 1.

**DeepZ/CROWN** The unstable ReLU bounds of DeepZ,  $\lambda x_{i-1,j}$  and  $\lambda x_{i-1,j} - \lambda l_{i-1,j}$  significantly increase the sensitivity. After the first ReLU layer, we have that  $x_{2,j}$  are in  $R_2(\delta)$ . This changes the behavior of all following linear layers, as a linear combination of  $M$  elements of  $R_N(\delta)$  is in  $R_{MN}(\delta)$ . Thus,  $x_{3,j} \in R_{2M}(\delta)$ . For the following ReLU layers, if we assume the inputs are in  $R_N(\delta)$ , we have that  $\lambda \in R_{2N}(\delta)$ , and thus the outputs are in  $R_{3N}(\delta)$ . Putting this together, each ReLU-linear block from layer 4 onwards multiplies the sensitivity by  $3M$ . As there are  $B \equiv \lceil L/2 \rceil - 1$  such blocks, we obtain  $2 \cdot 3^B M^{B+1}$  for the final sensitivity. CROWN uses the same upper ReLU bounds as DeepZ, so we can apply the same analysis, and show that the sensitivity of CROWN is  $2 \cdot 3^B M^{B+1}$  as well.

**CROWN-IBP** Here, at ReLU layer  $i$  during the (only) backsubstitution, we have to consider  $l_{i-1,j}$  and  $u_{i-1,j}$  separately from  $x_{i-1,j}$ . While the former were precomputed using Box, and are thus in  $P_1(\delta)$ , the latter get substituted as usual and can carry much larger sensitivity. Assuming  $x_{i-1,j} \in R_N(\delta)$  ( $N \geq 1$ ) and observing that we always have  $\lambda \in R_1(\delta)$ , it follows that  $x_{i,j} \in R_{N+1}(\delta)$ . As the linear layers have the same effect as before, each ReLU-linear block now increases the sensitivity from  $N$  to  $(N+1)M$ . As before,  $x_{3,j} \in R_{2M}(\delta)$ , so summing the geometric series that arises gives the final sensitivity of  $\frac{2M^{B+2} - M^{B+1} - M}{M-1}$ , which is in  $\mathcal{O}(M^{B+1})$ .

## 4.3 Can continuity and sensitivity be observed in practice?

To substantiate our theoretical results in practice, we train FC, a 5-layer network (see Appendix G), on MNIST using standard training. Then, we measure the change in the lower bound of one output neuron as we shift all first layer weights by  $\delta$  in the gradient direction of that output neuron. We show the resulting bounds depending on  $\delta$  in Figure 4, on a representative input with  $\epsilon = 0.15$ .

This confirms our results: hBox, CROWN, and CROWN-IBP indeed suffer from discontinuities, while Box and DeepZ do not. Compared to CROWN-IBP, CROWN uses the adaptive lower bound more often, introducing more discontinuities. While for hBox discontinuities appear only when  $l_{i-1,j} = 0$ , in CROWN they appear more often (see green line), namely whenever  $-l_{i-1,j} = u_{i-1,j}$ . While it is hard to visually notice sensitivity, we see that DeepZ is non-linear and Box is piecewise linear, both in line with our theory. We include more networks in Appendix E.

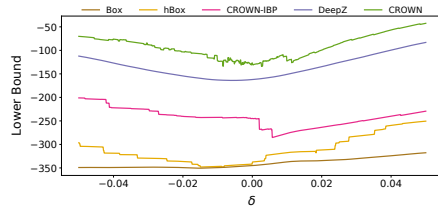

Figure 4: Discontinuity and sensitivity of relaxations on an MNIST FC network.

#### 4.4 How do continuity and sensitivity impact optimization?

Using both theoretical and empirical evidence, we have established that several common relaxations are discontinuous and highly sensitive. While in Section 5 we will experimentally confirm that these two properties negatively impact the success of certified training on real datasets, here we provide examples that can intuitively explain why these two properties affect gradient-based optimization. We consider a network with randomly sampled parameters and optimize first layer weights via standard gradient descent, trying to *maximize* the lower bound of one output neuron, produced using a particular relaxation. To plot the landscape in 1D, we restrict the optimization to the direction of the gradient in the initial point  $\delta = 0$  (as in Figure 4). We provide more details in Appendix F.

**The impact of discontinuities** The key issue with discontinuous relaxations (e.g., CROWN) is that gradient descent can fall off a cliff at a discontinuity in the landscape down to a region from which it fails to recover – i.e., where gradients do not lead it back, but to a suboptimal local maximum. We show a manifestation of this on a random network in Figure 5. Even though the landscape of CROWN allows for a higher global solution than Box, we can observe that gradient descent with CROWN drops at a discontinuity and converges to a worse objective value than Box. Continuous relaxations such as Box do not have this problem which allows gradient descent to easily navigate their optimization landscape. This is in line with observations in the literature that optimizing discontinuous functions requires more complex algorithms [36–38].

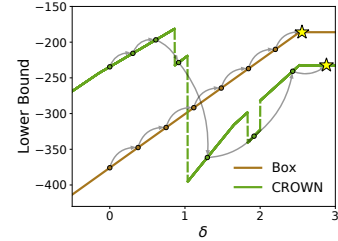

Figure 5: The impact of discontinuities: SGD obtains a looser bound with CROWN.

**The impact of high sensitivity** More sensitive relaxations (e.g. DeepZ) introduce a complex loss landscape with a larger number of local optima and saddle points, where gradient descent can often get stuck. An example is shown in Figure 6 where DeepZ has a highly non-linear landscape that traps gradient descent at a local maximum with a low objective value, not allowing it to progress to significantly better solutions on the right. Even though DeepZ is tighter for all  $\delta$ , Box has the lowest possible sensitivity and is thus piecewise linear, allowing gradient descent to quickly converge to a higher objective value. Furthermore, extensive theory [39–41] confirms that high-degree polynomial and rational functions, which we show appear for sensitive relaxations, are difficult to optimize. Note that sensitivity could be generalized beyond certified training to show that the training procedures used in common neural network setups have, like Box, the lowest possible sensitivity, implying that certified training with sensitive relaxations introduces an atypically complex landscape.

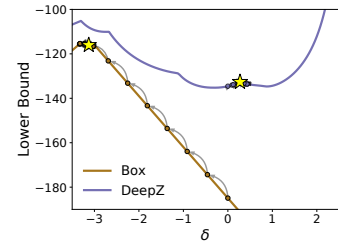

Figure 6: The impact of high sensitivity: SGD obtains a looser bound with DeepZ.

## 5 Experimental Evaluation

We now discuss our extensive experimental results. First, in Section 5.1, we evaluate certified training with convex relaxations and experimentally confirm our claims regarding the effect of continuity and sensitivity on training, resolving the paradox through the lens of these properties alongside tightness. Then, in Section 5.2 we provide a preliminary investigation into designing relaxations with favorable properties, via an experiment involving a novel training setup based on implicit layers [42, 43].

### 5.1 Resolving the paradox of certified training

We perform our experiments on the widely used datasets MNIST [44], FashionMNIST [45], SVHN [46], and CIFAR-10 [47]. To allow training with all relaxations introduced in Section 2, including time and memory intensive ones such as CROWN, we focus on two architectures: FC (a 5-layer fully-connected network) and CONV (a 3-layer convnet). On CIFAR-10, the accuracy of these networks is insufficient to obtain meaningful results, so we use a larger network CONV+ (a 4-layer convnet). Note that CROWN can not be run on networks as large as CONV+. Further increasing network size only marginally boosts all methods (see [1]). We provide architecture details in Appendix G.

Table 2: Evaluation of certified training with convex relaxations. We report certified accuracy (in %). For MNIST/FashionMNIST we use  $\epsilon_{test} = 0.3$ . For SVHN/CIFAR-10 we use  $\epsilon_{test} = 8/255$ .

| Method            | Tightness | Continuity | Sensitivity                | MNIST       |             | FashionMNIST |             | SVHN        | CIFAR-10    |
|-------------------|-----------|------------|----------------------------|-------------|-------------|--------------|-------------|-------------|-------------|
|                   |           |            |                            | FC          | CONV        | FC           | CONV        | CONV        | CONV+       |
| Box [2, 3, 7]     | low       | ✓          | $\mathcal{O}(1)$           | <b>74.0</b> | <b>86.8</b> | 40.4         | <b>52.0</b> | <b>28.9</b> | <b>29.0</b> |
| hBox [2, 8]       | mid       | ×          | $\mathcal{O}(1)$           | 57.0        | 83.7        | 39.6         | 47.1        | 23.6        | 20.0        |
| CROWN-IBP (R) [1] | mid       | ×          | $\mathcal{O}(M^{B+1})$     | 70.5        | 75.4        | <b>41.1</b>  | 40.0        | 27.5        | 24.3        |
| DeepZ [9–12]      | high      | ✓          | $\mathcal{O}(3^B M^{B+1})$ | 64.2        | 69.8        | 35.0         | 34.0        | 24.5        | 22.8        |
| CROWN [13, 14]    | high      | ×          | $\mathcal{O}(3^B M^{B+1})$ | 57.3        | 70.2        | 30.2         | 31.5        | 23.4        | OOM         |
| CROWN-IBP [1]     |           |            |                            | 77.9        | 86.6        | 47.9         | 50.9        | 29.3        | 30.3        |

We use the same relaxation for both training and certification, as this is most often optimal (see Appendix H). Orthogonal to our experiments are costly refinements of relaxations and MILP for certification, which could marginally improve the results. Finally, as our goal is to compare training with relaxations w.r.t. tightness, we separate CROWN-IBP from the main table as it is a hybrid approach combining CROWN-IBP (R) and IBP, with no clear way to define tightness. The training details are provided in Appendix G. All experiments use a single GeForce RTX 2080 Ti GPU.

**Resolving the paradox** Our main results are shown in Table 2 (more results can be found in Appendix I). Whereas prior work provided certain evidence, our comprehensive experiments over 5 relaxations, 4 datasets and several networks, confirm that the well known paradox of certified training generally holds: *tighter relaxations obtain worse results*.

To ease interpretation, we highlight for each relaxation when a property is favorable for training in green (high tightness, continuity, low sensitivity), and in yellow and red when it is progressively less favorable. Boundaries between favorability classes arise naturally; however, it is hard to make any statements about relaxations within one class for some property (e.g., which relaxation is tighter within a group), as well as quantify the relative impact of different properties on the result, as both of these might heavily depend on the setting (dataset, network, etc.).

Considering tightness as a sole property of a relaxation led to a seemingly contradictory conclusion. However, once we complement tightness with our two key properties, continuity and sensitivity, the results seem reasonable, as we are able to explain the inferior performance of each method compared to Box. Concretely, as we already established that discontinuity and sensitivity indeed manifest for realistic networks (Section 4.3), and explained the negative effect on gradient descent (Section 4.4), we can now expect that discontinuous and highly sensitive relaxations will not produce satisfactory results. This is confirmed in Table 2. Namely, we can attribute the poor results of hBox and CROWN-IBP (R) to the discontinuities in their loss landscape which harm gradient descent. While DeepZ does not suffer from discontinuities, its landscape is highly sensitive which again poses a difficulty for optimization and hurts the results. Notably, CROWN suffers from both issues, thus failing despite its tightness. We see that Box, while the least tight, has the most favorable continuity and sensitivity, and achieves the best results. This resolves the paradox, and directly replaces it with a clear explanation – *relaxations with unfavorable properties obtain worse results*.

## 5.2 Towards continuous, tight and non-sensitive relaxations

Our findings on the importance of continuity and sensitivity lead to deeper understanding of the developments in this field. Namely, the sole focus on tightness in the design of relaxations in prior work introduced complexity that as a side effect harmed continuity and sensitivity, outweighing the benefits of a tighter relaxation. For instance, while tightening the relaxation via an adaptive lower bound in CROWN improved certification, it created the discontinuity issue, leading to inferior results in training. A natural question then is: *is there a relaxation with all three favorable properties?*

**Triangle and Parallelogram** The most natural attempt would be to improve unfavorable properties of an existing relaxation. However, this is quite challenging, as improving a single property often negatively affects another property. For example, one way to make CROWN continuous is to, instead

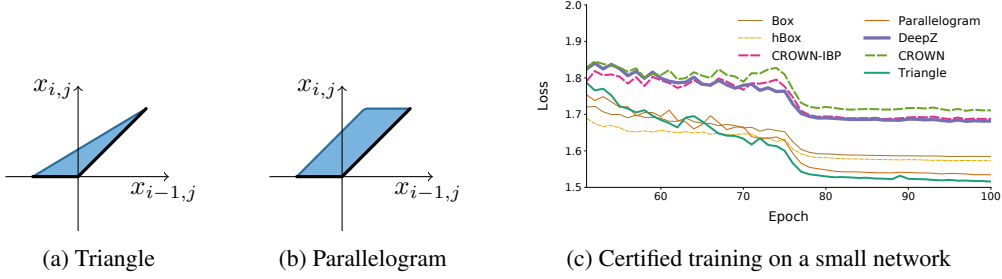

Figure 7: Training with new relaxations on a small network. Triangle and Parallelogram converge to a lower loss and achieve higher certified robustness than other relaxations.

of the adaptive choice, always use the lower bound  $x_{i,j} = 0$  (even for stable ReLUs). However, it is simple to check that this greatly harms tightness and plummets the performance in training (Appendix K). With this in mind, we turn to new relaxations, previously unused in training.

Interestingly, the tightest single neuron relaxation *Triangle* [48] (Figure 7a) is continuous, making it an attractive candidate for training. As it has no closed-form solution via backsubstitution, analyzing its sensitivity is challenging. However, as sensitivity intuitively arises from the slopes that depend on the bounds of previous layers, Triangle could have the sensitivity issues due to its upper bound. Replacing it with two upper bounds of constant slopes 0 and 1 yields a new relaxation, *Parallelogram* (Figure 7b). Even with such bounds, Parallelogram is still fairly tight (see Appendix B), continuous, and intuitively less sensitive. Continuity proofs for these relaxations can be found in Appendix D.2.

**Experiments with new relaxations** As already hinted, training with these relaxations has so far not been possible as computing the bounds requires solving a linear program. One attempt from prior work [49] was to learn the optimal slopes for CROWN (as this is provably as tight as Triangle [15]), but these slopes are difficult to find and the approach has not worked as well as Box. We show, for the first time, that both the Triangle and Parallelogram relaxations can be used for training small networks, leveraging recent advances in implicit optimization layers [42, 43] that enable differentiation through convex problems. Using *cvxpylayers* [43], we train a small  $2 \times 20$  network on a toy dataset. The details and full experimental results are given in Appendix K. The training loss of all methods for the last 50 epochs is shown in Figure 7c. While the performance of prior relaxations is consistent with our experiments on larger networks, Triangle and Parallelogram perform quite well: they achieve smaller losses than other relaxations and reach certified robustness of 52.4% and 52.3% (others fail to reach 50.5%). Note that we could not train larger networks due to high memory demands for training with Parallelogram or Triangle, but ongoing work in the area could improve this in the future [50, 51]. These results do not necessarily transfer to realistic networks and datasets, but they show that relaxations with favorable properties can achieve good results, supporting our previous claims.

### 5.3 Discussion and broader impact

We believe that our results aid future research by guiding the design of new relaxations with favorable properties. However, they could also uncover that training with convex relaxations is difficult, and that other methods such as randomized smoothing may be more promising. More broadly, while we do not anticipate any negative societal implications of our work, as convex relaxations have already been successfully applied in fairness research [52, 53] providing provable guarantees against individual discrimination, we believe our findings can indeed translate into a positive impact on society.

## 6 Conclusion

In this work we extensively reproduced and investigated the paradox of certified training, where tighter relaxations can obtain worse results. We identified two new properties: continuity and sensitivity of the loss, and used them alongside tightness to resolve the paradox. Based on these insights, we conducted a preliminary investigation in the design of relaxations with all favorable properties, using a novel experimental setup. We believe the insights of this work can help guide the design of new certified defenses and lead to a deeper understanding of this space.

## References

- [1] Huan Zhang, Hongge Chen, Chaowei Xiao, Sven Gowal, Robert Stanforth, Bo Li, Duane Boning, and Cho-Jui Hsieh. Towards stable and efficient training of verifiably robust neural networks. In *International Conference on Learning Representations*, 2020.
- [2] Matthew Mirman, Timon Gehr, and Martin Vechev. Differentiable abstract interpretation for provably robust neural networks. In *Proceedings of the 35th International Conference on Machine Learning*, 2018.
- [3] Sven Gowal, Krishnamurthy Dvijotham, Robert Stanforth, Rudy Bunel, Chongli Qin, Jonathan Uesato, Timothy Mann, and Pushmeet Kohli. On the effectiveness of interval bound propagation for training verifiably robust models. *arXiv preprint arXiv:1810.12715*, 2018.
- [4] Sven Gowal, Krishnamurthy Dvijotham, Robert Stanforth, Timothy Mann, and Pushmeet Kohli. A dual approach to verify and train deep networks. In *Proceedings of the Twenty-Eighth International Joint Conference on Artificial Intelligence, IJCAI-19*, 2019.
- [5] Mislav Balunovic and Martin Vechev. Adversarial training and provable defenses: Bridging the gap. In *International Conference on Learning Representations*, 2020.
- [6] Sungyoon Lee, Woojin Lee, Jinseong Park, and Jaewook Lee. Loss landscape matters: Training certifiably robust models with favorable loss landscape, 2021. URL <https://openreview.net/forum?id=lvXLfNeCQdK>.
- [7] Timon Gehr, Matthew Mirman, Dana Drachler-Cohen, Petar Tsankov, Swarat Chaudhuri, and Martin Vechev. Ai2: Safety and robustness certification of neural networks with abstract interpretation. In *2018 IEEE Symposium on Security and Privacy (S&P)*, 2018.
- [8] Shiqi Wang, Kexin Pei, Justin Whitehouse, Junfeng Yang, and Suman Jana. Formal security analysis of neural networks using symbolic intervals. In *USENIX Security Symposium*, pages 1599–1614. USENIX Association, 2018.
- [9] Eric Wong and Zico Kolter. Provable defenses against adversarial examples via the convex outer adversarial polytope. In *Proceedings of the 35th International Conference on Machine Learning*, 2018.
- [10] Gagandeep Singh, Timon Gehr, Matthew Mirman, Markus Püschel, and Martin Vechev. Fast and effective robustness certification. In *Advances in Neural Information Processing Systems 31*, 2018.
- [11] Lily Weng, Huan Zhang, Hongge Chen, Zhao Song, Cho-Jui Hsieh, Luca Daniel, Duane Boning, and Inderjit Dhillon. Towards fast computation of certified robustness for ReLU networks. In *Proceedings of the 35th International Conference on Machine Learning*, 2018.
- [12] Shiqi Wang, Kexin Pei, Justin Whitehouse, Junfeng Yang, and Suman Jana. Efficient formal safety analysis of neural networks. In *Advances in Neural Information Processing Systems 31*, 2018.
- [13] Huan Zhang, Tsui-Wei Weng, Pin-Yu Chen, Cho-Jui Hsieh, and Luca Daniel. Efficient neural network robustness certification with general activation functions. In *Advances in Neural Information Processing Systems 31*, 2018.
- [14] Gagandeep Singh, Timon Gehr, Markus Püschel, and Martin Vechev. An abstract domain for certifying neural networks. *Proceedings of the ACM on Programming Languages*, 2019.
- [15] Hadi Salman, Greg Yang, Huan Zhang, Cho-Jui Hsieh, and Pengchuan Zhang. A convex relaxation barrier to tight robustness verification of neural networks. In *Advances in Neural Information Processing Systems 32*, 2019.
- [16] Christian Szegedy, Wojciech Zaremba, Ilya Sutskever, Joan Bruna, Dumitru Erhan, Ian Goodfellow, and Rob Fergus. Intriguing properties of neural networks. *arXiv preprint arXiv:1312.6199*, 2013.

- [17] Battista Biggio, Igino Corona, Davide Maiorca, Blaine Nelson, Nedim Šrđić, Pavel Laskov, Giorgio Giacinto, and Fabio Roli. Evasion attacks against machine learning at test time. In *Joint European conference on machine learning and knowledge discovery in databases*, 2013.
- [18] Ian Goodfellow, Jonathon Shlens, and Christian Szegedy. Explaining and harnessing adversarial examples. In *International Conference on Learning Representations*, 2015.
- [19] Alexey Kurakin, Ian Goodfellow, and Samy Bengio. Adversarial machine learning at scale. *International Conference on Learning Representations*, 2017.
- [20] Aleksander Madry, Aleksandar Makelov, Ludwig Schmidt, Dimitris Tsipras, and Adrian Vladu. Towards deep learning models resistant to adversarial attacks. In *International Conference on Learning Representations*, 2018.
- [21] Aditi Raghunathan, Jacob Steinhardt, and Percy S Liang. Semidefinite relaxations for certifying robustness to adversarial examples. In *Advances in Neural Information Processing Systems 31*. 2018.
- [22] Sumanth Dathathri, Krishnamurthy Dvijotham, Alexey Kurakin, Aditi Raghunathan, Jonathan Uesato, Rudy Bunel, Shreya Shankar, Jacob Steinhardt, Ian J. Goodfellow, Percy Liang, and Pushmeet Kohli. Enabling certification of verification-agnostic networks via memory-efficient semidefinite programming. In *NeurIPS*, 2020.
- [23] François Serre, Christoph Müller, Gagandeep Singh, Markus Püschel, and Martin Vechev. Scaling polyhedral neural network verification on GPUs. In *Proc. Machine Learning and Systems (MLSys)*, 2021.
- [24] Mark Niklas Müller, Gleb Makarchuk, Gagandeep Singh, Markus Püschel, and Martin Vechev. Prima: Precise and general neural network certification via multi-neuron convex relaxations, 2021.
- [25] Shiqi Wang, Huan Zhang, Kaidi Xu, Xue Lin, Suman Jana, Cho-Jui Hsieh, and J. Zico Kolter. Beta-crown: Efficient bound propagation with per-neuron split constraints for complete and incomplete neural network verification. *CoRR*, abs/2103.06624, 2021.
- [26] Gagandeep Singh, Rupanshu Ganvir, Markus Püschel, and Martin Vechev. Beyond the single neuron convex barrier for neural network certification. In *Advances in Neural Information Processing Systems 32*, 2019.
- [27] Christian Tjandraatmadja, Ross Anderson, Joey Huchette, Will Ma, Krunal Patel, and Juan Pablo Vielma. The convex relaxation barrier, revisited: Tightened single-neuron relaxations for neural network verification. In *Advances in Neural Information Processing Systems 33*, 2020.
- [28] Guy Katz, Clark Barrett, David L Dill, Kyle Julian, and Mykel J Kochenderfer. Reluplex: An efficient smt solver for verifying deep neural networks. In *International Conference on Computer Aided Verification*, 2017.
- [29] Vincent Tjeng, Kai Y. Xiao, and Russ Tedrake. Evaluating robustness of neural networks with mixed integer programming. In *International Conference on Learning Representations*, 2019.
- [30] Jeremy Cohen, Elan Rosenfeld, and Zico Kolter. Certified adversarial robustness via randomized smoothing. In *Proceedings of the 36th International Conference on Machine Learning*, 2019.
- [31] Mathias Lecuyer, Vaggelis Atlidakis, Roxana Geambasu, Daniel Hsu, and Suman Jana. Certified robustness to adversarial examples with differential privacy. *2019 IEEE Symposium on Security and Privacy (S&P)*, 2018.
- [32] Hadi Salman, Greg Yang, Jerry Li, Pengchuan Zhang, Huan Zhang, Ilya Razenshteyn, and Sebastien Bubeck. Provably robust deep learning via adversarially trained smoothed classifiers. *Advances in Neural Information Processing Systems 32*, 2019.
- [33] Aditi Raghunathan, Jacob Steinhardt, and Percy Liang. Certified defenses against adversarial examples. In *International Conference on Learning Representations*, 2018.

- [34] Eric Wong, Frank Schmidt, Jan Hendrik Metzen, and J. Zico Kolter. Scaling provable adversarial defenses. In *Advances in Neural Information Processing Systems 31*. 2018.
- [35] Maximilian Baader, Matthew Mirman, and Martin T. Vechev. Universal approximation with certified networks. In *International Conference on Learning Representations*, 2020.
- [36] Andrew R Conn and Marcel Mongeau. Discontinuous piecewise linear optimization. *Mathematical programming*, 80(3):315–380, 1998.
- [37] José Mario Martínez. Minimization of discontinuous cost functions by smoothing. *Acta Applicandae Mathematica*, 71(3):245–260, 2002.
- [38] Achim Wechsung and Paul I Barton. Global optimization of bounded factorable functions with discontinuities. *Journal of Global Optimization*, 58(1):1–30, 2014.
- [39] Panos M Pardalos and Stephen A Vavasis. Quadratic programming with one negative eigenvalue is np-hard. *Journal of Global optimization*, 1(1):15–22, 1991.
- [40] Dorina Jibeteau and Etienne de Klerk. Global optimization of rational functions: a semidefinite programming approach. *Mathematical Programming*, 106(1):93–109, 2006.
- [41] MJ Valadan Zoej, Mehdi Mokhtarzade, Ali Mansourian, Hamid Ebadi, and S Sadeghian. Rational function optimization using genetic algorithms. *International journal of applied earth observation and geoinformation*, 9(4):403–413, 2007.
- [42] Brandon Amos and J. Zico Kolter. OptNet: Differentiable optimization as a layer in neural networks. In *Proceedings of the 34th International Conference on Machine Learning*, 2017.
- [43] A. Agrawal, B. Amos, S. Barratt, S. Boyd, S. Diamond, and Z. Kolter. Differentiable convex optimization layers. In *Advances in Neural Information Processing Systems 32*, 2019.
- [44] Y. Lecun, L. Bottou, Y. Bengio, and P. Haffner. Gradient-based learning applied to document recognition. *Proceedings of the IEEE*, 86(11):2278–2324, 1998. doi: 10.1109/5.726791.
- [45] Han Xiao, Kashif Rasul, and Roland Vollgraf. Fashion-mnist: a novel image dataset for benchmarking machine learning algorithms. *CoRR*, abs/1708.07747, 2017.
- [46] Yuval Netzer, Tao Wang, Adam Coates, Alessandro Bissacco, Bo Wu, and Andrew Y. Ng. Reading digits in natural images with unsupervised feature learning. In *NIPS Workshop on Deep Learning and Unsupervised Feature Learning 2011*, 2011. URL [http://ufldl.stanford.edu/housenumbers/nips2011\\_housenumbers.pdf](http://ufldl.stanford.edu/housenumbers/nips2011_housenumbers.pdf).
- [47] Alex Krizhevsky. Learning multiple layers of features from tiny images. Technical report, 2009.
- [48] Rüdiger Ehlers. Formal verification of piece-wise linear feed-forward neural networks. In *International Symposium on Automated Technology for Verification and Analysis*, 2017.
- [49] Sven Gowal, Krishnamurthy Dvijotham, Robert Stanforth, Timothy A Mann, and Pushmeet Kohli. A dual approach to verify and train deep networks. In *IJCAI*, 2019.
- [50] Quentin Berthet, Mathieu Blondel, Olivier Teboul, Marco Cuturi, Jean-Philippe Vert, and Francis Bach. Learning with differentiable perturbed optimizers. *arXiv preprint arXiv:2002.08676*, 2020.
- [51] Aaron Ferber, Bryan Wilder, Bistra Dilkina, and Milind Tambe. Mipaal: Mixed integer program as a layer. In *Proceedings of the AAAI Conference on Artificial Intelligence*, 2020.
- [52] Anian Ruoss, Mislav Balunovic, Marc Fischer, and Martin Vechev. Learning certified individually fair representations. In *Advances in Neural Information Processing Systems 33*. 2020.
- [53] Caterina Urban, Maria Christakis, Valentin Wüstholtz, and Fuyuan Zhang. Perfectly parallel fairness certification of neural networks. *Proc. ACM Program. Lang.*, 2020.
