# Supplementary material for: On the Paradox of Certified Training
Source: arXiv:2102.06700 source file (2022-10-12)
Supplement: Supplementary file 2 [file main_only_appendix.pdf]

# Supplementary Material

## A Backsubstitution example

Here we illustrate the process of backsubstitution concretely on the toy network shown in Figure 8, using the DeepZ relaxation. The same example but with the CROWN/DeepPoly relaxation is shown in [14].

The components of the input  $x_0$ , namely  $x_{0,1}$  and  $x_{0,2}$ , have bounds  $-1$  and  $1$ , meaning that  $-1 \leq x_{0,1}, x_{0,2} \leq 1$ . Because the first layer  $h_1$  is a linear layer we have

$$x_{1,1} = x_{0,1} + x_{0,2}, \quad (3)$$

$$x_{1,2} = x_{0,1} - x_{0,2}. \quad (4)$$

To obtain the bound  $l_{1,1}$  we replace both  $x_{0,1}$  and  $x_{0,2}$  with  $l_{0,1} = -1$  and  $l_{0,2} = -1$  as their signs are both positive in Equation 3 and obtain  $l_{1,1} = -2$ . To obtain  $l_{1,2}$  we replace  $x_{0,1}$  with  $l_{0,1} = -1$  and  $x_{0,2}$  with  $u_{0,1} = 1$  in Equation 4 as the sign of  $x_{0,2}$  is negative and obtain  $l_{1,2} = -2$ . Similarly we get  $u_{1,1} = 2$  and  $u_{1,2} = 2$ .

The second layer  $h_2$  is a ReLU layer. As both ReLUs are unstable, we need to calculate  $\lambda$  for each of them. As the bounds are equal,  $l_{1,1} = l_{1,2} = -2$  and  $u_{1,1} = u_{1,2} = 2$ , we get that  $\lambda$  is also equal,  $\lambda = \frac{1}{2}$ . Using the formula for unstable ReLUs we get

$$\begin{aligned} \frac{1}{2}x_{1,1} &\leq x_{2,1} \leq \frac{1}{2}x_{1,1} + 1, \\ \frac{1}{2}x_{1,2} &\leq x_{2,2} \leq \frac{1}{2}x_{1,2} + 1. \end{aligned}$$

Now backsubstituting the bounds for  $x_{0,1}$  and  $x_{0,2}$  gives

$$\begin{aligned} \frac{1}{2}(x_{0,1} + x_{0,2}) &\leq x_{2,1} \leq \frac{1}{2}(x_{0,1} + x_{0,2}) + 1, \\ \frac{1}{2}(x_{0,1} - x_{0,2}) &\leq x_{2,2} \leq \frac{1}{2}(x_{0,1} - x_{0,2}) + 1. \end{aligned}$$

The lower and upper bounds  $l_{2,1}, u_{2,1}$  and  $l_{2,2}, u_{2,2}$  for  $x_{2,1}$  and  $x_{2,2}$  respectively follow immediately

$$\begin{aligned} x_{2,1} &\geq \frac{1}{2}(l_{0,1} + l_{0,2}) = -1 = l_{2,1}, & x_{2,1} &\leq \frac{1}{2}(u_{0,1} + u_{0,2}) = 1 = u_{2,1}, \\ x_{2,2} &\geq \frac{1}{2}(l_{0,1} - u_{0,2}) = -1 = l_{2,2}, & x_{2,2} &\leq \frac{1}{2}(u_{0,1} - l_{0,2}) = 1 = u_{2,2}. \end{aligned}$$

The third layer  $h_3$  is again a linear layer, hence we get

$$\begin{aligned} x_{3,1} &= x_{2,1} + x_{2,2}, \\ x_{3,2} &= x_{2,1} - x_{2,2}. \end{aligned}$$

In the backsubstitution step, we replace  $x_{2,1}$  and  $x_{2,2}$  with their upper and lower bounds and arrive at

$$\begin{aligned} x_{0,1} &\leq x_{3,1} \leq x_{0,1} + 2, \\ x_{0,2} - 1 &\leq x_{3,2} \leq x_{0,2} + 1. \end{aligned}$$

Again, the lower and upper bounds  $l_{3,1}, u_{3,1}$  and  $l_{3,2}, u_{3,2}$  for  $x_{3,1}$  and  $x_{3,2}$  respectively follow

$$\begin{aligned} x_{3,1} &\geq l_{0,1} = -1 = l_{3,1}, \\ x_{3,1} &\leq u_{0,1} + 2 = 3 = u_{3,1}, \\ x_{3,2} &\geq l_{0,2} - 1 = -2 = l_{3,2}, \\ x_{3,2} &\leq u_{0,2} + 1 = 2 = u_{3,2}. \end{aligned}$$

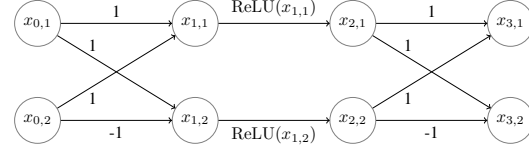

Figure 8: Toy network (from Singh et al. [14]).

Table 3: The summary of tightness experiments. Robustness is evaluated using PGD with the same radius  $\epsilon$  used in training.

| Experiment | Dataset      | Network  | Training             | Accuracy (%) | Robustness (%) |
|------------|--------------|----------|----------------------|--------------|----------------|
| A          | MNIST        | CONV     | Standard             | 98.7         | /              |
| B          | MNIST        | CONV     | PGD $\epsilon = 0.1$ | 99.0         | 94.4           |
| C          | MNIST        | CONV     | PGD $\epsilon = 0.3$ | 98.2         | 91.0           |
| D          | FashionMNIST | CONV     | Standard             | 91.4         | /              |
| E          | CIFAR-10     | CONV+    | Standard             | 70.0         | /              |
| F          | MNIST        | FC-SMALL | Standard             | 98.2         | /              |
| G          | MNIST        | FC-SMALL | PGD $\epsilon = 0.1$ | 99.0         | 91.8           |
| H          | MNIST        | FC-SMALL | PGD $\epsilon = 0.3$ | 92.3         | 78.3           |

## B Tightness experiments

In this section, we show the full results of our tightness experiments, one of which (experiment A) was shown in Table 1 and Figure 2.

**Setup** We conduct 8 experiments (labeled A-H), varying the dataset (MNIST, FashionMNIST, CIFAR-10), the network (CONV and CONV+, described in Appendix G, and FC-SMALL, a 100-100-10 fully-connected network), and the training method (standard training, adversarial training with PGD with  $\epsilon = 0.1$ , and adversarial training with PGD with  $\epsilon = 0.3$ ). We use FC-SMALL to be able to include Triangle and Parallelogram, relaxations introduced in Section 5.2. For PGD, we use 100 steps with step size 0.01. We train all models for 200 epochs. For PGD with  $\epsilon = 0.3$ , as necessary for convergence, we use the first 10 epochs as warm-up (standard training), and the following 50 as ramp-up, where we slowly increase the perturbation radius from 0 to  $\epsilon$ . We use L2 regularization with strength  $5e-3$  for experiment E, and  $5e-5$  for other experiments. The experiments are summarized in Table 3.

After training the networks, we sample 100  $\epsilon$  values from 0 to 0.07 for standard, 0 to 0.15 for PGD  $\epsilon = 0.1$ , and 0 to 0.4 for PGD  $\epsilon = 0.3$  models. For every radius  $\epsilon$ , we use each convex relaxation to attempt to certify the examples from the test set. For experiments A-E we use all test set examples, while for F-H we use the first 100, as LP-based relaxations (Triangle and Parallelogram) are computationally intensive. We calculate the certified robustness of each network under all relaxations, and plot the resulting CR curves. The CR curves shown in Figure 2 show the results of experiment A. Additionally, we provide the CR curves for experiment F in Figure 9, to enable visual inspection of the tightness of Triangle and Parallelogram (discussed later in this section).

Further, we quantify the tightness of each relaxation as CR-AUC, the area under the CR curve, calculated using the trapezoidal rule. Table 1 contains CR-AUC values of the curves from Figure 2 (experiment A), and the certified robustness after certified training of the same network with  $\epsilon_{train} = 0.3$  (an excerpt from the full results given in Section 5.1).

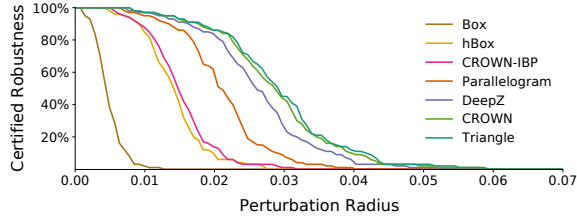

Figure 9: CR curves in tightness experiment F.

**Discussion** As the curves are similar among experiments, we summarize the results (CR-AUC) for all experiments in Table 4. From these results, we can confirm two claims given in the main paper:

*It is necessary to use certified training to obtain a certifiably robust network.* We can see that adversarial training, along with improving empirical robustness, also has a positive effect on certified robustness. However, these results are significantly worse from those that can be obtained using certified training. To illustrate this point, for experiment C (MNIST, CONV, PGD with  $\epsilon = 0.3$ ), the method that certifies the most at  $\epsilon = 0.3$  is CROWN, with 11.9% certified robustness (not visible from the results shown here). Using certified training in the same setting, *all* relaxations obtain significantly better results: from 69.8% (worst method) to 86.8% (best method), as seen in Table 2.

Table 4: The results of tightness experiments (A-H), showing CR-AUC of each method. We include the tightness classes as in Table 2.

| Method        | Tightness | A    | B    | C     | D    | E    | F    | G    | H     |
|---------------|-----------|------|------|-------|------|------|------|------|-------|
| Box           | low       | 0.73 | 0.91 | 1.94  | 0.20 | 0.02 | 0.47 | 0.63 | 2.22  |
| hBox          | mid       | 1.76 | 4.76 | 10.45 | 0.53 | 0.09 | 1.42 | 2.70 | 11.44 |
| CROWN-IBP     | mid       | 2.15 | 4.20 | 8.85  | 0.70 | 0.04 | 1.50 | 2.73 | 13.55 |
| DeepZ         | high      | 3.00 | 9.21 | 20.97 | 1.11 | 0.25 | 2.63 | 6.21 | 21.57 |
| CROWN         | high      | 3.36 | 9.77 | 22.75 | 1.19 | 0.28 | 2.86 | 6.74 | 22.63 |
| Triangle      |           |      |      |       |      |      | 2.92 | 6.87 | 25.53 |
| Parallelogram |           |      |      |       |      |      | 2.10 | 4.58 | 22.81 |

The relative tightness of relaxations is well established and can be empirically confirmed. More concretely, we can see that the grouping of relaxations in three “tightness classes”, as originally shown in Table 2, indeed naturally arises from the results, and is consistent across all our experiments. We further see that Triangle, as the theoretically optimal single-neuron ReLU relaxation, is always the tightest. Interestingly, Parallelogram is fairly tight, with its CR-AUC always between the two more favorable tightness classes.

## C hBox certifies more than Box

Here we prove that for any neural network parameters hBox certifies more than Box:

**Theorem 2** (Informal). *Given a neural network architecture parametrized by  $\theta \in \mathbb{R}^d$ , for any choice of  $\theta$ , hBox can certify robust classification for more inputs than Box.*

*Proof.* For a formal proof see [8] or [2]. To prove the statement, it is sufficient to show that the constraints introduced for each layer for hBox are tighter than Box constraints. This is relatively straightforward for linear layers, so here we focus on ReLU layers. For unstable ReLU both use the same constraints:  $0 \leq x_{i,j} \leq u_{i-1,j}$ . When  $u_{i-1,j} < 0$ , both set  $x_{i,j} = 0$ . The only difference is when  $l_{i-1,j} > 0$ : in this case Box uses  $l_{i-1,j} \leq x_{i,j} \leq u_{i-1,j}$ , while hBox sets  $x_{i,j} = x_{i-1,j}$ . By definition we have  $l_{i-1,j} \leq x_{i-1,j} \leq u_{i-1,j}$ , implying that hBox constraints are indeed tighter.  $\square$

## D Continuity proofs

In this section we provide continuity proofs for Box, DeepZ, Triangle and Parallelogram.

### D.1 Proof for Box and DeepZ

Here we expand on the proof sketch given in the main paper to provide a complete proof of Theorem 1.

**Proof. Box:** Recall that for Box,  $l_i$  and  $u_i$  are computed directly as a function of  $l_{i-1}$ ,  $u_{i-1}$ , and  $\theta$ . For linear layers, this function is a sum of products of elements in  $l_{i-1}$ ,  $u_{i-1}$  and  $\theta$ , which is continuous w.r.t. all variables. If  $i$  is a ReLU layer, the lower (upper) bound function is  $\text{ReLU}(l_{i-1,j})$  (resp.  $\text{ReLU}(u_{i-1,j})$ ), which is also clearly continuous. As compositions, sums, and products of continuous functions are continuous functions, this directly shows that  $l_{L,j}$  are ultimately continuous.

**DeepZ:** For DeepZ, the computation of each  $l_i$  and  $u_i$  includes backsubstitution, where to obtain the final expressions (as in Equation 2), we repeatedly substitute in lower/upper bound expressions, based on the values of  $\theta$  and  $l_{i'}$  and  $u_{i'}$  from all previous layers. Note that as before, it suffices to show that for some  $i$ ,  $l_i$  and  $u_i$  are continuous w.r.t.  $\theta$  and all previous  $l_{i'}$  and  $u_{i'}$ .

First, recall that during each step of backsubstitution we encounter terms of the form  $\alpha \cdot x_{i',j}$ , and based on the sign of  $\alpha$  substitute the lower or the upper bound expression for  $x_{i',j}$ . When one such  $\alpha = 0$ ,  $\alpha \cdot x_{i',j}$  is continuous (both the left and the right limit equal the function value at that point,

0). Thus, we can reduce these cases to cases where no  $\alpha$  values encountered are zero, i.e., all choices for the upper/lower bound to be substituted during backsubstitution are *fixed*.

Next, recall that even if we fix this choice, the actual expression we substitute in for the upper or lower bound may depend on the ReLU stability case. If all  $l_{i'}$  and  $u_{i'}$  are nonzero the stability is fixed, and by substituting linear and ReLU relaxation bounds during backsubstitution we can arrive at a closed form expression w.r.t.  $\theta$  that uses only elementary operations, which is continuous.

It is left to discuss the behavior in points where some elements of some  $l_{i'}$  or  $u_{i'}$  are zero. In this case the ReLU is still stable, but switches to being unstable on one side of zero. If  $l_{i',j} = 0$  both upper and lower bound expressions for  $x_{i'+1,j}$  are  $x_{i',j}$ , which is also the right limit. In the left limit, we use the unstable ReLU bounds  $\lambda x_{i',j}$  and  $\lambda x_{i',j} - \lambda l_{i',j}$  and see that for  $l_{i',j} \rightarrow 0$ ,  $\lambda \rightarrow 1$ , and thus these bounds approach  $x_{i',j}$  as well, so there is no discontinuity. Similarly, for  $u_{i',j} = 0$  (the other stable case) the bounds (as well as the left limit) are 0. For the right limit, we again have the unstable case, but now  $\lambda \rightarrow 0$ , so both bounds approach 0, implying that this is also not a discontinuity.

To conclude, we showed that  $l_i$  and  $u_i$  are continuous w.r.t.  $\theta$  and all previous  $l_{i'}$  and  $u_{i'}$ . This can be composed to conclude that  $l_{L,j}$  is continuous w.r.t.  $\theta$ , using the same argument we used for Box.  $\square$

## D.2 Proof for Triangle and Parallelogram

Here we state and prove a similar theorem for additional relaxations introduced in Section 5.2.

**Theorem 3.** *The final layer bounds  $l_{L,j}$  produced by Triangle and Parallelogram are continuous functions with respect to  $\theta$ .*

*Proof.* We proceed inductively, layer by layer, in  $i$ -th step proving the continuity of  $l_i$  and  $u_i$  with respect to  $\theta_{1:i-1}$ ,  $l_{1:i-1}$  and  $u_{1:i-1}$ . As described in more details later in Appendix K:

$$\begin{aligned} l_{i,j} &:= \min x_{i,j}, & \text{subject to: } \mathbf{Ax} = \mathbf{b}, \mathbf{Gx} \leq \mathbf{h} \\ u_{i,j} &:= \max x_{i,j}, & \text{subject to: } \mathbf{Ax} = \mathbf{b}, \mathbf{Gx} \leq \mathbf{h}. \end{aligned}$$

Note that  $\mathbf{A}$ ,  $\mathbf{G}$ ,  $\mathbf{b}$  and  $\mathbf{h}$  are functions of  $\theta_{1:i-1}$ ,  $l_{1:i-1}$  and  $u_{1:i-1}$ , but we omit this from the notation for brevity. Each inductive step of the proof consists of two parts.

First, we prove that  $\mathbf{A}$ ,  $\mathbf{G}$ ,  $\mathbf{b}$  and  $\mathbf{h}$  are continuous functions of  $\theta_{1:i-1}$ ,  $l_{1:i-1}$  and  $u_{1:i-1}$ . We will prove continuity for each type of equality and inequality separately. If  $x_{i,j}$  is a linear function of  $x_{i-1}$ , then rows of  $\mathbf{A}$  and  $\mathbf{b}$  corresponding to this equality are simply weights of the network which are by definition continuous with respect to the weights. Next, we consider inequalities which make up the rows of  $\mathbf{G}$  and  $\mathbf{h}$ . If  $x_{i,j} = \text{ReLU}(x_{i-1,j})$ , then both Triangle and Parallelogram add two lower bounds  $x_{i,j} \geq 0$  and  $x_{i,j} \geq x_{i-1,j}$ . These clearly do not depend on any of the weights  $\theta_{1:i-1}$  or bounds  $l_{1:i-1}$  and  $u_{1:i-1}$ , and are thus trivially continuous with respect to them. When considering the upper bounds of the Parallelogram,  $x_{i,j} \leq u_{i-1,j}$ ,  $x_i \leq x_{i-1,j} - l_{i-1,j}$ , it is easy to check the continuity in cases when  $u_{i-1,j} \rightarrow 0$  or  $l_{i-1,j} \rightarrow 0$ . It remains to consider the upper bound of Triangle,  $x_{i,j} \leq \lambda_{i,j} x_{i-1,j} - \lambda_{i,j} l_{i,j}$  where  $\lambda_{i,j} = u_{i-1,j} / (u_{i-1,j} - l_{i-1,j})$ . The argument is the same as the one used to prove the continuity of DeepZ: if we let  $l_{i-1,j} \rightarrow 0$ , then  $\lambda_{i,j} \rightarrow 1$  and if we let  $u_{i-1,j} \rightarrow 0$ , then  $\lambda_{i,j} \rightarrow 0$  which recovers the bounds for  $l_{i-1,j} \geq 0$  and  $u_{i-1,j} \leq 0$ , respectively.

In the second part of the proof, consider the Lagrangian dual of the linear program for  $l_{i,j}$ ,

$$\mathcal{L}(\mathbf{x}, \boldsymbol{\mu}, \boldsymbol{\lambda}, \theta_{1:i-1}, l_{1:i-1}, u_{1:i-1}) = x_{i,j} + \sum_{k=1}^{n_{eq}} \mu_k (\mathbf{a}_k^T \mathbf{x} - b_k) + \sum_{k=1}^{n_{ineq}} \lambda_k (\mathbf{g}_k^T \mathbf{x} - h_k)$$

where  $\mathbf{a}_k$ ,  $b_k$ ,  $\mathbf{g}_k$ ,  $h_k$  all depend on  $\theta_{1:i-1}$ ,  $l_{1:i-1}$ ,  $u_{1:i-1}$ , but we do not show this explicitly. Moreover, they depend on them in a continuous way, as shown earlier. This means that  $\mathcal{L}$ , as a composition of continuous functions, is continuous. Based on strong duality of the original linear program (see e.g., Salman et al. [15]) we know that

$$l_{i,j}(\theta_{1:i-1}, l_{1:i-1}, u_{1:i-1}) = \max_{\lambda \geq 0, \boldsymbol{\mu}} \min_{\mathbf{x} \in \mathcal{D}} \mathcal{L}(\mathbf{x}, \boldsymbol{\mu}, \boldsymbol{\lambda}, \theta_{1:i-1}, l_{1:i-1}, u_{1:i-1}).$$

where  $\mathcal{D}$  is the compact domain which bounds each  $x_{i,j}$  by its interval bounds. Taking minimum or maximum over a coordinate results in a continuous function (can be shown using basic calculus), and the composition of continuous functions is continuous which is enough to prove the claim.

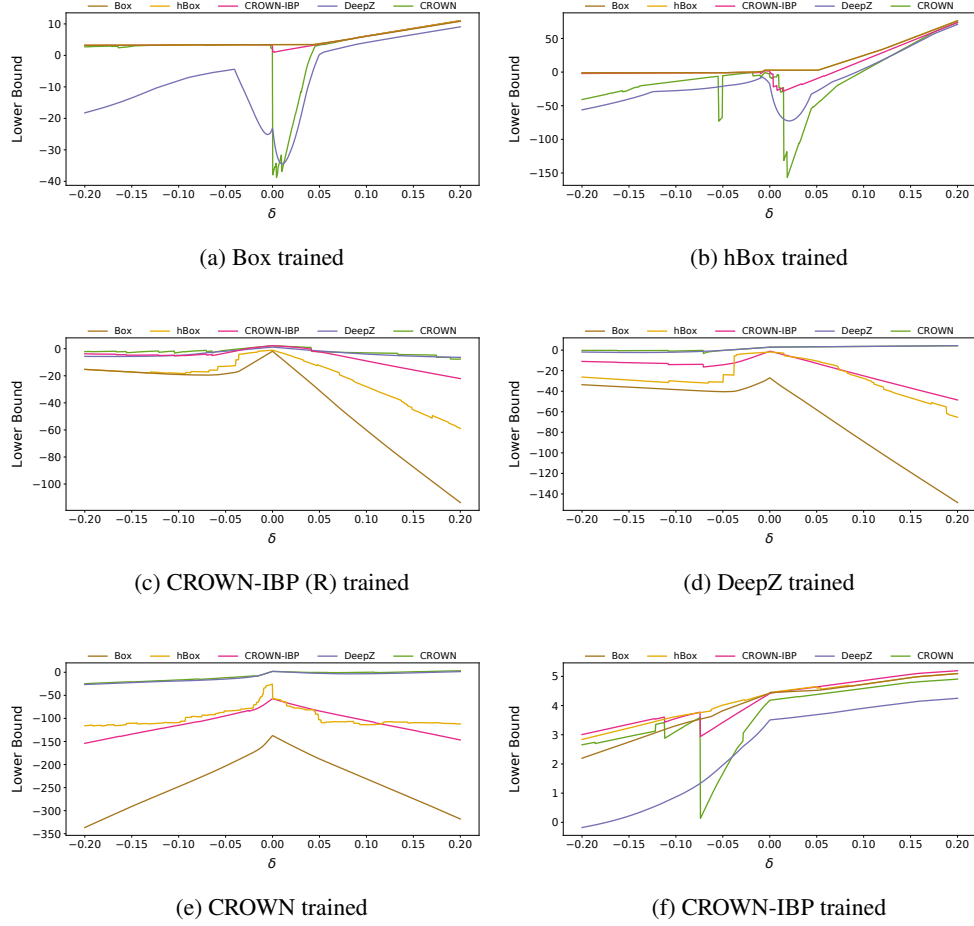

Figure 10: Lower bounds of convex relaxations for 6 MNIST FC networks from Table 2 with  $\epsilon = \epsilon_{test} = 0.3$ , showing continuity and sensitivity of each relaxation. Each subfigure shows the name of the relaxation used to train the corresponding network.

Finally, as we can prove the claim for each step of the induction, we obtain the proof that  $l_{L,j}$  are continuous with respect to  $\theta$ .

□

## E Additional figures showing continuity and sensitivity in practice

Here we show additional figures for continuity and sensitivity with the same setup as for Figure 4. In Figure 10 we show the bounds obtained for each of the MNIST FC networks from Table 2, using  $\epsilon = \epsilon_{test} = 0.3$ . Note that each network is trained using a different relaxation. All plots are generated on the same example. We can highlight some differences compared to the naturally trained network. First, as explained earlier, the relaxation used for training typically obtains the tightest bounds. Next, we can see that if the network was trained with CROWN or hBox, there is a significantly smaller number of discontinuities than in the cases when the network was trained naturally or using some other relaxation. Even though there is a lack of discontinuities in these cases, these networks do not perform well (see Table 2) which suggests that, while the network learned to eliminate the discontinuities, the performance was still hurt by them earlier in the training. Finally, we see that evaluating Box and hBox trained models using the DeepZ relaxation shows its increased sensitivity.

Table 5: The architectures used in our main experiments. “FC  $n$ ” denotes a fully-connected layer with  $n$  neurons. “CONV  $k\ w \times h + s$ ” denotes a convolutional layer with  $k$  kernels of size  $w \times h$  and stride  $s$ . All activations are ReLU. CONV+ is equivalent to „small” in Gowal et al. [3].

| FC     | CONV          | CONV+         |
|--------|---------------|---------------|
| FC 400 | CONV 16 4x4+2 | CONV 16 4x4+2 |
| FC 200 | FC 100        | CONV 32 4x4+1 |
| FC 100 | FC 10         | FC 100        |
| FC 100 |               | FC 10         |
| FC 10  |               |               |

## F Details of experiments with SGD in 4.4

In this section we provide details of the experiments used to generate Figure 5 and Figure 6. For both examples we consider an architecture consisting of 2 hidden layers with 10 neurons each, and 2 output neurons. The network receives a 1-dimensional input. We randomly sample the input, weights, and biases as integers between -4 and 4, and we sample the perturbation radius  $\epsilon$  between 0.1 and 4.1.

For the experiment with the discontinuous CROWN relaxation, we set the initial learning rate to 0.02, learning rate decay to 0.99, and ran for 20 epochs. For the experiment with the sensitive DeepZ relaxation, we set the initial learning rate to 0.005, learning rate decay to 0.99, and ran for 100 epochs. We sampled a number of different networks for both scenarios, and chose the one which best illustrates the behavior of gradient descent.

## G Details of the main experiments

Here we detail the setup of the main experiments shown in Table 2. The details of network architectures FC, CONV, and CONV+ are shown in Table 5. The training parameters vary by dataset.

For MNIST, we tune all hyperparameters thoroughly. We train all models for 200 epochs, starting with a *warm-up* ( $N_w$  epochs) followed by a *ramp-up* period ( $N_r$  epochs) to stabilize the training procedure [3]. During the warm-up we train the network naturally. During the ramp-up we gradually increase the perturbation radius  $\epsilon$  from 0 to  $\epsilon_{train}$ , decrease  $\kappa$  from  $\kappa_{start} = 1$  to  $\kappa_{end}$  (shifting from natural to certified training), and for CROWN-IBP gradually shift from CROWN-IBP (R) to IBP loss. We use a batch size of 100 (50 for memory intensive models) and train using the Adam optimizer with the initial learning rate  $\alpha$ . Finally, we use  $L_1$  regularization with the strength hyperparameter  $\lambda$ . We tune  $(N_w, N_r, \kappa_{end}, \lambda, \alpha)$ , as well as the learning rate schedule (*milestones*, where we reduce the learning rate  $10\times$  at epochs 130 and 190, or *steps*, where we halve it every 20 epochs), and the choice of last layer elision (where we elide the final layer  $h_L$  of the network with the specifications  $c_{y'}$  as in Gowal et al. [3]). For each perturbation radius  $\epsilon_{test} \in \{0.1, 0.2, 0.3\}$ , we train with  $\epsilon_{train} \in \{0.1, 0.2, 0.3, 0.4\}$  and report the best result. In Table 6 we show the best choice of hyperparameters for each model used in our evaluation (see Appendix I for complete results).

For FashionMNIST, we reuse the best hyperparameter choice of the corresponding MNIST model.

For SVHN, we use the parameters given in prior work as a starting point, and introduce minimal changes. For Box, CROWN-IBP (R), and CROWN-IBP, we start from the parameters given in Gowal et al. [3]: we train for 2200 epochs with batch size 50, warm-up for 10 epochs, ramp-up for 1100 epochs, use Adam with initial learning rate of  $\alpha = 1e-3$  (reduced  $10\times$  at 60% and 90% of the training steps), and use  $\epsilon_{train} = 1.1\epsilon_{test}$ . We do not use random translations (as we notice these harm the results on large  $\epsilon_{test}$ ), and we tune  $\kappa_{end}$  (trying 0 and 0.5 for each method – 0 performs better for all methods except CROWN-IBP (R)), introduce L1 regularization (improves the results only for Box, with  $\lambda = 5e-5$ ), tune the initial learning rate (we end up using  $\alpha = 5e-4$  or Box and CROWN-IBP). For hBox, DeepZ and CROWN, we use the parameters from Wong and Kolter [9]: batch size of 20, training for 100 epochs (training longer does not improve the results), using Adam with initial learning rate  $\alpha = 1e-3$  halved every 10 epochs, ramp-up w.r.t.  $\epsilon$  of 50 epochs where we start from  $\epsilon = 0.001$ . We introduce ramp-up w.r.t.  $\kappa$  with  $\kappa_{end} = 0$ . As before, we exclude the data transformations. For all three methods we use L1 regularization with  $\lambda = 5e-6$ .

Table 6: The best choice of hyperparameters for each MNIST model in our evaluation.

| Net  | $\epsilon_{test}$ | Method        | $\epsilon_{train}$ | $N_w$ | $N_r$ | $\kappa_{end}$ | $\lambda$ | $\alpha$ | LR schedule | Elision |
|------|-------------------|---------------|--------------------|-------|-------|----------------|-----------|----------|-------------|---------|
| FC   | 0.1               | Box           | 0.2                | 10    | 100   | 0.5            | 5e-6      | 5e-4     | milestones  | yes     |
| FC   | 0.2               | Box           | 0.2                | 10    | 100   | 0              | 5e-6      | 5e-4     | milestones  | yes     |
| FC   | 0.3               | Box           | 0.3                | 10    | 100   | 0              | 5e-6      | 5e-4     | milestones  | yes     |
| FC   | 0.1               | hBox          | 0.1                | 0     | 50    | 0              | 5e-5      | 5e-4     | milestones  | yes     |
| FC   | 0.2               | hBox          | 0.2                | 10    | 50    | 0.5            | 5e-5      | 5e-4     | milestones  | yes     |
| FC   | 0.3               | hBox          | 0.3                | 0     | 50    | 0.5            | 5e-5      | 5e-4     | milestones  | yes     |
| FC   | 0.1               | CROWN-IBP (R) | 0.2                | 0     | 50    | 0.5            | 5e-6      | 5e-4     | milestones  | yes     |
| FC   | 0.2               | CROWN-IBP (R) | 0.3                | 0     | 50    | 0.5            | 5e-6      | 5e-4     | milestones  | yes     |
| FC   | 0.3               | CROWN-IBP (R) | 0.3                | 0     | 50    | 0.5            | 5e-6      | 5e-4     | milestones  | yes     |
| FC   | 0.1               | DeepZ         | 0.1                | 10    | 50    | 0              | 5e-6      | 5e-4     | milestones  | yes     |
| FC   | 0.2               | DeepZ         | 0.2                | 0     | 50    | 0              | 5e-6      | 1e-3     | steps       | no      |
| FC   | 0.3               | DeepZ         | 0.3                | 0     | 50    | 0              | 5e-6      | 1e-3     | steps       | no      |
| FC   | 0.1               | CROWN         | 0.1                | 0     | 100   | 0              | 0         | 5e-4     | milestones  | yes     |
| FC   | 0.2               | CROWN         | 0.2                | 10    | 50    | 0              | 0         | 5e-4     | milestones  | yes     |
| FC   | 0.3               | CROWN         | 0.3                | 10    | 100   | 0              | 0         | 5e-4     | milestones  | yes     |
| FC   | 0.1               | CROWN-IBP     | 0.2                | 10    | 50    | 0.5            | 0         | 5e-4     | milestones  | yes     |
| FC   | 0.2               | CROWN-IBP     | 0.2                | 10    | 50    | 0              | 0         | 5e-4     | milestones  | yes     |
| FC   | 0.3               | CROWN-IBP     | 0.3                | 10    | 100   | 0              | 0         | 5e-4     | milestones  | yes     |
| CONV | 0.1               | Box           | 0.2                | 0     | 50    | 0.5            | 5e-6      | 5e-4     | milestones  | yes     |
| CONV | 0.2               | Box           | 0.3                | 0     | 50    | 0.5            | 5e-6      | 5e-4     | milestones  | yes     |
| CONV | 0.3               | Box           | 0.3                | 0     | 50    | 0.5            | 5e-6      | 5e-4     | milestones  | yes     |
| CONV | 0.1               | hBox          | 0.3                | 0     | 50    | 0.5            | 5e-5      | 5e-4     | milestones  | yes     |
| CONV | 0.2               | hBox          | 0.3                | 0     | 50    | 0.5            | 5e-5      | 5e-4     | milestones  | yes     |
| CONV | 0.3               | hBox          | 0.3                | 0     | 50    | 0.5            | 5e-5      | 5e-4     | milestones  | yes     |
| CONV | 0.1               | CROWN-IBP (R) | 0.1                | 10    | 50    | 0              | 0         | 5e-4     | milestones  | yes     |
| CONV | 0.2               | CROWN-IBP (R) | 0.2                | 10    | 50    | 0              | 0         | 5e-4     | milestones  | yes     |
| CONV | 0.3               | CROWN-IBP (R) | 0.3                | 10    | 50    | 0.5            | 5e-6      | 5e-4     | milestones  | yes     |
| CONV | 0.1               | DeepZ         | 0.2                | 0     | 50    | 0              | 5e-6      | 5e-4     | milestones  | yes     |
| CONV | 0.2               | DeepZ         | 0.2                | 0     | 50    | 0              | 5e-6      | 5e-4     | milestones  | yes     |
| CONV | 0.3               | DeepZ         | 0.3                | 0     | 50    | 0              | 5e-5      | 5e-4     | milestones  | yes     |
| CONV | 0.1               | CROWN         | 0.2                | 10    | 100   | 0              | 0         | 5e-4     | milestones  | yes     |
| CONV | 0.2               | CROWN         | 0.2                | 10    | 100   | 0              | 0         | 5e-4     | milestones  | yes     |
| CONV | 0.3               | CROWN         | 0.3                | 10    | 100   | 0              | 0         | 5e-4     | milestones  | yes     |
| CONV | 0.1               | CROWN-IBP     | 0.2                | 10    | 100   | 0.5            | 5e-6      | 5e-4     | milestones  | yes     |
| CONV | 0.2               | CROWN-IBP     | 0.3                | 10    | 50    | 0.5            | 5e-6      | 5e-4     | milestones  | yes     |
| CONV | 0.3               | CROWN-IBP     | 0.3                | 10    | 50    | 0              | 5e-6      | 5e-4     | milestones  | yes     |

For CIFAR-10, we similarly use the parameters from prior work. For Box, CROWN-IBP (R), and CROWN-IBP, we use the values from Zhang et al. [1]: 3200 epochs, 320 of warm-up and 1600 of ramp-up (using  $\kappa_{end} = 0$  and  $\epsilon_{train} = 1.1\epsilon_{test}$  for all methods,  $\kappa_{start} = 1$  for Box and  $\kappa_{start} = 0$  for other methods), Adam with  $\alpha = 5e-4$  reduced  $10\times$  at epochs 2600 and 3040, and random horizontal flips and crops as augmentation. We halve the batch size to 512 for all three methods. For DeepZ and hBox we use 50 random Cauchy projections [34] and the parameters based on Wong et al. [34] but with extended training length and introduced ramp-up w.r.t.  $\kappa$ : we train with batch size 50 for 240 epochs, 80 of which are ramp-up, using Adam optimizer with  $\alpha = 5e-4$ , halved every 10 epochs. During ramp-up we start from  $\epsilon = 0.001$ , and use  $\kappa_{start} = 1$  and  $\kappa_{end} = 0$ .

## H Training and certifying with different relaxations

In this section, we investigate the effect of varying the convex relaxation based method used to certify a network trained using some method  $\mathcal{M}$ . We use the MNIST models with  $\epsilon_{test} = 0.3$  from Table 2 and the corresponding models for  $\epsilon_{test} = 0.1$  from the full results given in Appendix I, on both FC and CONV architectures. We evaluate their certified robustness using all five introduced methods. The results are given in Table 7. Observe that almost all Box trained models have extremely



Table 7: The evaluation of models trained with certified training using different convex relaxations.

| Net  | $\epsilon_{test}$ | Method (training) | Method (certification) |      |           |       |             |
|------|-------------------|-------------------|------------------------|------|-----------|-------|-------------|
|      |                   |                   | Box                    | hBox | CROWN-IBP | DeepZ | CROWN       |
| FC   | 0.1               | Box               | 89.5                   | 89.5 | 84.1      | 44.7  | 67          |
| FC   | 0.3               | Box               | 74                     | 74   | 64.5      | 3.7   | 25.5        |
| FC   | 0.1               | hBox              | 88.4                   | 88.4 | 83.4      | 36.6  | 55.9        |
| FC   | 0.3               | hBox              | 57                     | 57   | 10.8      | 2.4   | 7.1         |
| FC   | 0.1               | CROWN-IBP (R)     | 5.7                    | 76.8 | 90.6      | 90.2  | 90.5        |
| FC   | 0.3               | CROWN-IBP (R)     | 1.8                    | 10.4 | 70.5      | 37.4  | 56.8        |
| FC   | 0.1               | DeepZ             | 0                      | 0.1  | 0.6       | 92.5  | <b>93</b>   |
| FC   | 0.3               | DeepZ             | 0                      | 0.1  | 1.8       | 64.2  | 63.5        |
| FC   | 0.1               | CROWN             | 0                      | 0    | 0         | 90.9  | 91.6        |
| FC   | 0.3               | CROWN             | 0                      | 0    | 0         | 54.3  | 57.3        |
| FC   | 0.1               | CROWN-IBP         | 91.2                   | 91.2 | 88.2      | 65.3  | 78.2        |
| FC   | 0.3               | CROWN-IBP         | 77.9                   | 77.9 | 72.6      | 8.6   | 29          |
| CONV | 0.1               | Box               | 94.6                   | 94.7 | 93.1      | 92.3  | 92.9        |
| CONV | 0.3               | Box               | 86.8                   | 86.8 | 64.9      | 12.4  | 46.7        |
| CONV | 0.1               | hBox              | 92.7                   | 92.7 | 91.7      | 90.6  | 91.2        |
| CONV | 0.3               | hBox              | 83.7                   | 83.7 | 73.4      | 26.3  | 50.3        |
| CONV | 0.1               | CROWN-IBP (R)     | 0                      | 59.1 | 93.4      | 93.1  | 93.5        |
| CONV | 0.3               | CROWN-IBP (R)     | 0                      | 0.2  | 75.4      | 59.5  | 67.6        |
| CONV | 0.1               | DeepZ             | 12                     | 92.6 | 94.7      | 94.9  | <b>95.1</b> |
| CONV | 0.3               | DeepZ             | 0.4                    | 25.8 | 60.9      | 69.8  | <b>74</b>   |
| CONV | 0.1               | CROWN             | 0.1                    | 87.8 | 93.6      | 94.4  | 94.5        |
| CONV | 0.3               | CROWN             | 0                      | 0.3  | 55.1      | 65.2  | 70.2        |
| CONV | 0.1               | CROWN-IBP         | 94.4                   | 94.5 | 93.3      | 92.4  | 92.9        |
| CONV | 0.3               | CROWN-IBP         | 86.6                   | 86.6 | 78        | 32.8  | 60.3        |

low certified robustness when certified with DeepZ, even though it is tighter, and vice versa. This confirms our previous statement that training with  $\mathcal{M}$  produces a network particularly suitable to certification with  $\mathcal{M}$ , and justifies our decision to focus on this case. The few exceptions, i.e., the instances where a method different than  $\mathcal{M}$  achieved a better result (by more than the minimal 0.1% after rounding), are marked in bold. We can see that certification with tighter CROWN often slightly improves DeepZ-trained networks. However, this improvement mostly leaves the relative order of methods unchanged and does not affect our conclusions. Note that if we are interested in the highest certified robustness of an already trained model, the best approach is to always use more expensive certifiers [29, 26, 27] which are not fast enough to be used in training. However, in this work we focus on analyzing the training properties of a single relaxation, and not on maximizing the certified robustness.

## I Complete results of the main experiments

In Tables 8 to 12 we present complete certified training evaluation results, expanding the ones given in Section 5.1. In all tables, Acc denotes accuracy, PGD denotes empirical robustness against PGD attacks (we use 100 steps with step size 0.01), and CR denotes certified robustness. For MNIST/FashionMNIST datasets we include two smaller perturbation radii,  $\epsilon_{test} = 0.1$  and  $\epsilon_{test} = 0.2$ . Note that the paradox of certified training can rarely be observed for such small radii. To explain the unusually high *standard accuracy* of CROWN-IBP (R) in our CIFAR-10 experiments, note that it is the only method that performs better with  $\kappa_{end} = 0.5$  (as opposed to  $\kappa_{end} = 0$ ). All other methods could reach similar standard accuracy with  $\kappa_{end} = 0.5$ , but their certified accuracy would drop.



Table 8: Complete evaluation results on the MNIST dataset with the FC network.

| Method        | $\epsilon_{test} = 0.1$ |         |        | $\epsilon_{test} = 0.2$ |         |        | $\epsilon_{test} = 0.3$ |         |        |
|---------------|-------------------------|---------|--------|-------------------------|---------|--------|-------------------------|---------|--------|
|               | Acc (%)                 | PGD (%) | CR (%) | Acc (%)                 | PGD (%) | CR (%) | Acc (%)                 | PGD (%) | CR (%) |
| Box           | 94.8                    | 90.7    | 89.5   | 92.6                    | 86.6    | 82.4   | 88.7                    | 80.8    | 74.0   |
| hBox          | 95.6                    | 90.6    | 88.4   | 93.2                    | 82.1    | 76.6   | 89.2                    | 65.7    | 57.0   |
| CROWN-IBP (R) | 94.9                    | 91.8    | 90.6   | 92.2                    | 84.6    | 80.9   | 92.2                    | 79.9    | 70.5   |
| DeepZ         | 98.3                    | 95.1    | 92.5   | 95.0                    | 90.9    | 85.1   | 87.4                    | 77.9    | 64.2   |
| CROWN         | 98.6                    | 94.6    | 91.6   | 93.0                    | 85.5    | 80.6   | 84.9                    | 71.7    | 57.3   |
| CROWN-IBP     | 95.5                    | 92.0    | 91.2   | 93.3                    | 88.6    | 86.0   | 90.8                    | 83.6    | 77.9   |

Table 9: Complete evaluation results on the MNIST dataset with the CONV network.

| Method        | $\epsilon_{test} = 0.1$ |         |        | $\epsilon_{test} = 0.2$ |         |        | $\epsilon_{test} = 0.3$ |         |        |
|---------------|-------------------------|---------|--------|-------------------------|---------|--------|-------------------------|---------|--------|
|               | Acc (%)                 | PGD (%) | CR (%) | Acc (%)                 | PGD (%) | CR (%) | Acc (%)                 | PGD (%) | CR (%) |
| Box           | 97.2                    | 95.0    | 94.6   | 95.9                    | 92.3    | 91.3   | 95.9                    | 89.7    | 86.8   |
| hBox          | 95.1                    | 93.0    | 92.7   | 95.1                    | 90.9    | 89.5   | 95.1                    | 87.9    | 83.7   |
| CROWN-IBP (R) | 98.5                    | 95.2    | 93.4   | 95.5                    | 90.9    | 86.9   | 93.4                    | 84.5    | 75.4   |
| DeepZ         | 97.0                    | 95.7    | 94.9   | 97.0                    | 94.0    | 88.8   | 92.5                    | 87.0    | 69.8   |
| CROWN         | 96.8                    | 95.1    | 94.5   | 96.8                    | 92.6    | 88.0   | 92.6                    | 84.3    | 70.2   |
| CROWN-IBP     | 96.9                    | 94.8    | 94.4   | 95.6                    | 92.0    | 90.9   | 94.8                    | 89.1    | 86.6   |

Table 10: Complete evaluation results on the FashionMNIST dataset with the FC network.

| Method        | $\epsilon_{test} = 0.1$ |         |        | $\epsilon_{test} = 0.2$ |         |        | $\epsilon_{test} = 0.3$ |         |        |
|---------------|-------------------------|---------|--------|-------------------------|---------|--------|-------------------------|---------|--------|
|               | Acc (%)                 | PGD (%) | CR (%) | Acc (%)                 | PGD (%) | CR (%) | Acc (%)                 | PGD (%) | CR (%) |
| Box           | 79.2                    | 71.4    | 67.9   | 73.7                    | 65.2    | 57.9   | 54.8                    | 46.6    | 40.4   |
| hBox          | 79.2                    | 73.1    | 70.0   | 76.3                    | 62.5    | 56.4   | 68.7                    | 49.2    | 39.6   |
| CROWN-IBP (R) | 76.6                    | 68.1    | 66.5   | 69.6                    | 54.7    | 51.3   | 69.6                    | 46.7    | 41.1   |
| DeepZ         | 81.2                    | 73.7    | 70.2   | 71.2                    | 57.6    | 51.6   | 51.0                    | 39.2    | 35.0   |
| CROWN         | 80.8                    | 70.6    | 67.8   | 70.9                    | 53.7    | 49.5   | 52.4                    | 35.9    | 30.2   |
| CROWN-IBP     | 78.1                    | 72.1    | 69.6   | 74.7                    | 64.7    | 58.9   | 66.7                    | 55.9    | 47.9   |

Table 11: Complete evaluation results on the FashionMNIST dataset with the CONV network.

| Method        | $\epsilon_{test} = 0.1$ |         |        | $\epsilon_{test} = 0.2$ |         |        | $\epsilon_{test} = 0.3$ |         |        |
|---------------|-------------------------|---------|--------|-------------------------|---------|--------|-------------------------|---------|--------|
|               | Acc (%)                 | PGD (%) | CR (%) | Acc (%)                 | PGD (%) | CR (%) | Acc (%)                 | PGD (%) | CR (%) |
| Box           | 80.3                    | 74.1    | 72.7   | 76.5                    | 65.5    | 61.4   | 76.5                    | 58.8    | 52.0   |
| hBox          | 72.9                    | 67.0    | 65.2   | 72.9                    | 61.3    | 57.4   | 72.9                    | 53.6    | 47.1   |
| CROWN-IBP (R) | 81.0                    | 72.5    | 69.9   | 71.8                    | 58.2    | 54.5   | 68.9                    | 50.2    | 40.0   |
| DeepZ         | 72.3                    | 66.6    | 64.8   | 72.3                    | 60.1    | 53.4   | 56.3                    | 40.7    | 34.0   |
| CROWN         | 71.9                    | 64.3    | 62.8   | 71.9                    | 55.2    | 49.4   | 56.4                    | 39.9    | 31.5   |
| CROWN-IBP     | 80.0                    | 73.5    | 72.1   | 74.7                    | 63.7    | 60.2   | 65.3                    | 56.5    | 50.9   |

Table 12: Complete evaluation results on SVHN dataset with the CONV network and  $\epsilon_{test} = 8/255$  (left), and on CIFAR-10 dataset with the CONV+ network and  $\epsilon_{test} = 8/255$  (right).

| Method        | Acc (%) | PGD (%) | CR (%) | Method        | Acc (%) | PGD (%) | CR (%) |
|---------------|---------|---------|--------|---------------|---------|---------|--------|
| Box           | 41.6    | 30.9    | 28.9   | Box           | 39.8    | 32.4    | 29.0   |
| hBox          | 35.0    | 26.9    | 23.6   | hBox          | 36.2    | 25.9    | 20.0   |
| CROWN-IBP (R) | 65.8    | 37.2    | 27.5   | CROWN-IBP (R) | 37.4    | 28.7    | 24.3   |
| DeepZ         | 38.7    | 27.7    | 24.5   | DeepZ         | 36.5    | 28.6    | 22.8   |
| CROWN         | 44.0    | 27.3    | 23.4   | CROWN         | OOM     | OOM     | OOM    |
| CROWN-IBP     | 43.9    | 32.6    | 29.3   | CROWN-IBP     | 41.1    | 32.8    | 30.3   |

Table 13: The variability of the results when changing the seed.

| Dataset      | Net  | Seed |      |      |      |      |      |      |      |      |      | Mean | Stddev |
|--------------|------|------|------|------|------|------|------|------|------|------|------|------|--------|
|              |      | 10   | 11   | 12   | 13   | 14   | 15   | 16   | 17   | 18   | 19   |      |        |
| MNIST        | FC   | 74   | 70.8 | 70.6 | 71.5 | 70.9 | 69.9 | 72.7 | 72.2 | 65   | 69   | 70.7 | 2.45   |
| MNIST        | CONV | 86.8 | 86.6 | 85.7 | 86.5 | 86.1 | 86.2 | 86.1 | 85.4 | 86.3 | 85   | 86.1 | 0.56   |
| FashionMNIST | FC   | 40.4 | 40.4 | 38.8 | 40.6 | 42.1 | 39.8 | 45   | 42.5 | 42.6 | 42.7 | 41.5 | 1.82   |
| FashionMNIST | CONV | 52   | 51.7 | 51   | 50   | 52.1 | 51.6 | 50.2 | 50.4 | 52.1 | 52.2 | 51.3 | 0.86   |

## J Estimating the effect of the seed

To estimate variability and demonstrate that it does not significantly impact our main conclusions, we use one efficient method (Box) and perform the same run with best parameters from Appendix G with 10 seed values, across two datasets (MNIST and FashionMNIST) and both networks (FC and CONV). In all experiments we use  $\epsilon_{test} = 0.3$ . The results, with the mean and the standard deviation of obtained results, are given in Table 13. Note that, for both MNIST networks, the results we report in Table 2 are the best out of all 10 seeds (74% and 86.8% respectively), as expected given that the hyperparameters were tuned on this seed. As is it too expensive to run repetitions for relaxations other than Box, we can not estimate the confidence intervals of their results. Nonetheless, if we took the confidence interval of the size of two standard deviations for our Box results, it would not change the conclusions we made based on single experiment runs reported in Table 2. Namely, continuity and sensitivity, alongside tightness, can explain the results in Table 2.

## K Details of our experiments in Section 5.2

In this section we describe the encodings of several commonly used convex relaxations as linear programs. We provide a general version of the encoding which was used in Section 5.2 to train with Triangle and Parallelogram, but it can also be used to train with all other linear relaxations that we introduced in this work, using encodings described in Appendix K.2. Further, we provide experimental details for our experiments with Triangle and Parallelogram and elaborate on the claims made in Section 5.2 regarding attempts to improve CROWN by making it continuous.

### K.1 Training Triangle and Parallelogram with implicit layers

Here we give a formal encoding of Triangle and Parallelogram, and describe how to train with them using the framework of implicit layers.

**Relaxation via a Linear Program (LP)** Consider a relaxation that sequentially processes the layers and the neurons at each layer. For one neuron, we collect all current linear constraints and construct an LP which is then minimized and maximized to compute the scalar lower and upper bounds of this neuron. The upper bound of neuron  $j$  at layer  $i$  is defined as a solution of an LP,

$$u_{i,j} := \max x_{i,j}, \quad \text{subject to: } \mathbf{Ax} = \mathbf{b}, \mathbf{Gx} \leq \mathbf{h}. \quad (5)$$

Here  $\mathbf{A}, \mathbf{G}, \mathbf{b}$  and  $\mathbf{h}$  are all functions of the parameters  $\theta_{1:i-1}$  and the neuron bounds  $\mathbf{l}_{1:i-1}$  and  $\mathbf{u}_{1:i-1}$ , of the previous layers. As these bounds are themselves the results of optimization problems, the overall computation can be characterized as a multi-level optimization problem. This general formulation captures all relaxations introduced in Section 2, with their particular formulations shown in Appendix K.2, but here we use them only for Triangle and Parallelogram.

**Triangle and Parallelogram** The Triangle relaxation of ReLU is formally defined as:

$$\begin{aligned} x_{i,j} &\geq 0, & x_{i,j} &\geq x_{i-1,j}, \\ x_{i,j} &\leq x_{i-1,j} \cdot u / (u - l) - ul / (u - l), \end{aligned}$$

where we set  $l \equiv l_{i-1,j}$  and  $u \equiv u_{i-1,j}$ . Parallelogram relaxation of ReLU is determined by the following constraints:

$$\begin{aligned} x_{i,j} &\geq 0, & x_i &\geq x_{i-1,j} \\ x_{i,j} &\leq u, & x_i &\leq x_{i-1,j} - l \end{aligned}$$

## K.2 LP encodings of common relaxations

**Box** If layer  $i$  is a linear function  $\mathbf{x}_i = \mathbf{W}_i \mathbf{x}_{i-1} + \mathbf{b}_i$ , then we add the inequality constraint  $x_{i,j} \leq (\mathbf{W}_{i,j})^T \mathbf{x}_{i-1}^U + b_{i,j}$  where  $x_{i-1,k}^U = u_{i-1,k}$  if  $W_{i,j,k}$  is positive and  $l_{i-1,k}$  otherwise. Similarly, we add the inequality constraint  $x_{i,j} \geq (\mathbf{W}_{i,j})^T \mathbf{x}_{i-1}^L + b_{i,j}$  where  $x_{i-1,k}^L = l_{i-1,k}$  if  $W_{i,j,k}$  is positive and  $u_{i-1,k}$  otherwise. If layer  $i$  is the ReLU activation function  $\mathbf{x}_i = \text{ReLU}(\mathbf{x}_{i-1})$ , then we add inequality constraints  $x_{i,j} \leq \max(0, u_{i-1,j})$  and  $x_{i,j} \geq \max(0, l_{i-1,j})$ .

**DeepZ** If layer  $i$  is a linear function  $\mathbf{x}_i = \mathbf{W}_i \mathbf{x}_{i-1} + \mathbf{b}_i$ , then we simply add the equality constraint  $\mathbf{x}_i = \mathbf{W}_i \mathbf{x}_{i-1} + \mathbf{b}_i$ . If layer  $i$  is the ReLU activation function  $\mathbf{x}_i = \text{ReLU}(\mathbf{x}_{i-1})$ , then we add the equality constraint  $x_{i,j} = \lambda_{i,j} x_{i-1,j} + \mu_{i,j} + \mu_{i,j} e_{i,j}$ . Here,  $e_{i,j}$  is an auxiliary variable assuming values between -1 and 1 (thus it requires two additional inequality constraints  $e_{i,j} \leq 1$  and  $e_{i,j} \geq -1$ ). Coefficients  $\lambda_{i,j}$  and  $\mu_{i,j}$  are defined as follows, distinguishing three cases based on whether  $x_{i-1,j}$  crosses zero: (i)  $u_{i-1,j} \leq 0$ , in which case  $\lambda_{i,j} = 0$  and  $\mu_{i,j} = 0$ ; (ii)  $l_{i-1,j} \geq 0$ , in which case  $\lambda_{i,j} = 1$  and  $\mu_{i,j} = 0$ ; and (iii)  $l_{i-1,j} < 0 < u_{i-1,j}$ , in which case  $\lambda_{i,j} = u_{i-1,j} / (u_{i-1,j} - l_{i-1,j})$  and  $\mu_{i,j} = -\frac{1}{2} l_{i-1,j} u_{i-1,j} / (u_{i-1,j} - l_{i-1,j})$ . Note that here we define auxiliary variables  $e_{i,j}$ , but we could express an equivalent linear program (to respect the notation used in Equation 5) without them by substituting  $\mu_{i,j} e_{i,j} = x_{i,j} - \lambda_{i,j} x_{i-1,j} - \mu_{i,j}$ .

**CROWN** If layer  $i$  is a linear function  $\mathbf{x}_i = \mathbf{W}_i \mathbf{x}_{i-1} + \mathbf{b}_i$ , then we simply add the equality constraint  $\mathbf{x}_i = \mathbf{W}_i \mathbf{x}_{i-1} + \mathbf{b}_i$ . If layer  $i$  is the ReLU activation function  $\mathbf{x}_i = \text{ReLU}(\mathbf{x}_{i-1})$ , then we distinguish three cases based on whether  $x_{i-1,j}$  crosses zero: (i)  $u_{i-1,j} \leq 0$ , in which case we add the equality constraint  $x_{i,j} = 0$ ; (ii)  $l_{i-1,j} \geq 0$ , in which case we add the equality constraint  $x_{i,j} = x_{i-1,j}$ ; and (iii)  $l_{i-1,j} < 0 < u_{i-1,j}$ , in which case we add two inequality constraints, one for the lower bound and one for the upper bound. The upper bound constraint is given as  $x_{i,j} \leq \frac{u_{i-1,j}}{u_{i-1,j} - l_{i-1,j}} x_{i-1,j} - \frac{l_{i-1,j} u_{i-1,j}}{u_{i-1,j} - l_{i-1,j}}$ . The lower bound constraint is set to  $x_{i,j} \geq 0$  if  $-l_{i-1,j} > u_{i-1,j}$ , and otherwise it is set to  $x_{i,j} \geq x_{i-1,j}$ .

## K.3 Details of the experiment with Triangle and Parallelogram

Here we provide more details on the experiment conducted in Section 5.2. We train a small network with 2 layers, both consisting of 20 hidden neurons. For our dataset, we apply PCA to 1024 random samples of the MNIST dataset, to obtain 16-dimensional inputs. We train with all previously introduced relaxations, and compare them to Triangle and Parallelogram. To train with LP relaxations, we use the `cvxpylayers` library [43] and PyTorch [54]. For all relaxations we use  $\epsilon_{\text{train}} = 0.3$ , and train with batch size 64 for 10 warm-up epochs, followed by 50 ramp-up epochs and 50 standard epochs. We choose the same hyperparameters for all relaxations. Figure 7c shows the loss of all methods during the last 50 epochs of training. Table 14 shows the standard and certified robustness of all models after training.

Table 14: Results of our experiment with Triangle and Parallelogram.

| Method        | Acc (%) | CR (%) |
|---------------|---------|--------|
| Box           | 72.27   | 49.12  |
| hBox          | 68.85   | 50.29  |
| CROWN-IBP (R) | 76.37   | 46.88  |
| DeepZ         | 75.78   | 50.49  |
| CROWN         | 75.59   | 44.14  |
| Triangle      | 73.34   | 52.44  |
| Parallelogram | 72.75   | 52.25  |

## K.4 Performance of CROWN-0

To demonstrate that improving unfavorable properties of existing relaxations is challenging, we introduce CROWN-0, a modification of CROWN that removes the discontinuity issue by replacing the adaptive lower bound with the fixed lower bound  $x_{i,j} \geq 0$ . We implement this variant and add it to several of the tightness experiments given in Appendix B. In all our runs, with the usual resolution for sampling  $\epsilon$ , CROWN-0 obtains CR-AUC of 0. This demonstrates that by making the relaxation continuous we greatly sacrificed tightness. Further, we attempt to use CROWN-0 in certified training but are, as expected given our conclusions about tightness, unable to obtain meaningful results.
